# Supplementary material for: LCLS in - photon out: fluorescence measurement of neon using soft x-rays
Source: arXiv:1708.01283 source file (2017-08-03)
Supplement: Supplementary file 1 [file Supplementary_Data_neon_expt_photon_yields.pdf]

```
Get["NeonRateEquations.m", Path -> NotebookDirectory[]]
```

```
HartreeToeV := 27.2113845
eVToHartree := 1 / HartreeToeV
JouleToHartree := 2.29371269*^17
MilliJouleToHartree := 1*^-3 * JouleToHartree
BohrToAngstroem := 0.5291772083
AngstroemToBohr := 1 / BohrToAngstroem
MicrometerToBohr := 1*^4 * AngstroemToBohr
BohrToMicrometer := 1 / MicrometerToBohr
t0ToSecond := 24.18884326505*^-18
t0ToFemtoSecond := 24.18884326505*^-3
FemtoSecondTot0 :=  1 / t0ToFemtoSecond
crossSectionAUtoBarn := 1*^8 * BohrToAngstroem ^ 2
crossSectionAUtocm2 := crossSectionAUtoBarn * 1*^-24
crossSectioncm2toAU := 1 / crossSectionAUtocm2
intensityAUtoSI := 6.436409085121321*^15
intensitySItoAU := 1 / intensityAUtoSI
```

```
neginfinity := -10 000 / t0ToFemtoSecond
posinfinity := 10 000 / t0ToFemtoSecond
```

# Fluorescence from a neon atom in LCLS radiation

Christian Buth, 12 July 2017

Theoretische Chemie, Physikalisch-Chemisches Institut, Ruprecht-Karls-Universität Heidelberg, Im Neuenheimer Feld 229, 69120 Heidelberg, Germany

## LCLS x-ray pulse

### Temporal profile

LCLS photon energy:

```
omegaX := 1200 * eVToHartree
```

LCLS FWHM pulse duration:

```
tauX := 100 * FemtoSecondTot0
```

LCLS beamline transmission loss and actual pulse energy:

```
optdamp := 0.5
pulseenergy := optdamp * 1.2 * MilliJouleToHartree
```

LCLS peak fluence:

```
J0X := 2 * Sqrt[Log[2] / Pi] * 8*^11 / (1*^4 / BohrToAngstroem) ^2 / tauX
```

Gaussian x-ray flux pulse shape (See Eq. (7) in Ref. [1]):

```
jxgaussian[J0Xj_, tX_, t_] := J0Xj * Exp[-4 * Log[2] * (t / tX) ^2] * UnitStep[t + 2 * tX] * UnitStep[2 * tX - t]
flux[t_] := jxgaussian[J0X, tauX, t]
```

```
Plot[{flux[t / t0ToFemtoSecond], 1 / 2 * flux[0] * UnitStep[t / t0ToFemtoSecond + tauX / 2] * UnitStep[tauX / 2 - t / t0ToFemtoSecond]},
 {t, -200, 200}, PlotStyle → {{Red, Thick}, {Green, Thick}}, PlotRange → All]
```

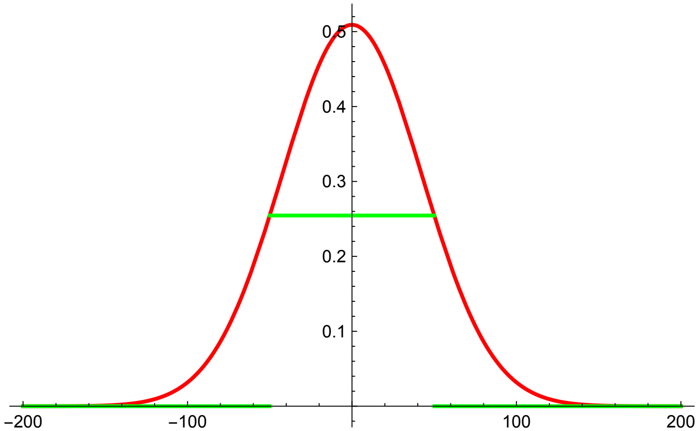


## Crater profile

The crater is normalized to unity with respect to an integration over the whole xy plane:

```
craterX[rx_]:=1/rhoXx/Sqrt[Pi/Log[16]]*Exp[-4*Log[2]*(rx/rhoXx)^2]
craterY[ry_]:=1/rhoYy/Sqrt[Pi/Log[16]]*Exp[-4*Log[2]*(ry/rhoYy)^2]
crater[rx_,ry_]:=craterX[rx]*craterY[ry]
```

Number of radial integration points for the crater integration:

```
nintdata:=100
```

## Fluence profile

Number of x-ray photons for “monochromatic” light pulses:

```
numXRays[pulseenergy_,photonenergy_]:=pulseenergy/photonenergy
```

X-ray fluence, i.e., the number of photos per squaremeter:

```
fluence[pulseenergy_,photonenergy_,rx_,ry_]:=numXRays[pulseenergy,photonenergy]*crater[rx,ry]
```

```
peakfluence[pulseenergy_,photonenergy_]:=fluence[pulseenergy,photonenergy,0,0]
```

The peak x-ray flux at a point in the beam area:

```
J0Xfun[pulseenergy_,photonenergy_,tauX_,rx_,ry_]:=2*Sqrt[Log[2]/Pi]/tauX*fluence[pulseenergy,photonenergy,rx,ry]
```

Gaussian x-ray flux pluse shape:

```
jxgaussian[J0Xj_,tX_,t_]:=J0Xj*Exp[-4*Log[2]*(t/tX)^2]*UnitStep[t+2*tX]*UnitStep[2*tX-t]
```

# Radiative decay of certain configurations

```
idxconfig = <|Table[configurations[[i]] → i, {i, 1, Length[configurations]}]|>
```

```
<|226 → 1, 225 → 2, 216 → 3, 126 → 4, 224 → 5, 215 → 6, 206 → 7, 125 → 8, 116 → 9, 026 → 10, 223 → 11, 214 → 12, 205 → 13, 124 → 14,
 115 → 15, 106 → 16, 025 → 17, 016 → 18, 222 → 19, 213 → 20, 204 → 21, 123 → 22, 114 → 23, 105 → 24, 024 → 25, 015 → 26, 006 → 27,
 221 → 28, 212 → 29, 203 → 30, 122 → 31, 113 → 32, 104 → 33, 023 → 34, 014 → 35, 005 → 36, 220 → 37, 211 → 38, 202 → 39,
 121 → 40, 112 → 41, 103 → 42, 022 → 43, 013 → 44, 004 → 45, 210 → 46, 201 → 47, 120 → 48, 111 → 49, 102 → 50, 021 → 51,
 012 → 52, 003 → 53, 200 → 54, 110 → 55, 101 → 56, 020 → 57, 011 → 58, 002 → 59, 100 → 60, 010 → 61, 001 → 62, 000 → 63|>
```

```
terminalcfg = Map[idxconfig, {"226", "225", "224", "223", "222", "221", "220", "210", "200", "100", "000"}]
```

```
{1, 2, 5, 11, 19, 28, 37, 46, 54, 60, 63}
```

## Configurations which decay exclusively radiatively

```
Table[If[! existsGamAtot[[i]] && existsGamRtot[[i]], configurations[[i]], ""], {i, 1, Length[existsGamAtot]}]
```

```
{, , 216, , , 215, 206, , , , , 214, 205, , , , , , , 213, 204, , , , , , , ,
 212, 203, , , , , , , , 211, 202, , , , , , , , 201, , , , , , , , 110, 101, , , , , 010, 001, }
```

```
{GamRTot216, GamRTot215, GamRTot206, GamRTot214, GamRTot205, GamRTot213, GamRTot204, GamRTot212,
  GamRTot203, GamRTot211, GamRTot202, GamRTot201, GamRTot110, GamRTot101, GamRTot010, GamRTot001} * posinfinity
```

{0.201701, 0.161539, 0.191075, 0.115628, 0.147279, 0.071781, 0.0989526, 0.0360639,
0.0556178, 0.0119578, 0.0237782, 0.00585518, $7.44227\times 10^{-8}$, 23.3024, $2.51004\times 10^{-7}$, 62.5627}

```
1 / GamRTot110 * t0ToSecond * 1*^6
```

```
134.368
```

```
{GamATot126, GamATot125, GamATot124, GamATot123, GamATot122, GamATot121,
  GamATot116, GamATot115, GamATot114, GamATot113, GamATot112, GamATot111,
  GamATot106, GamATot105, GamATot104, GamATot103, GamATot102} * posinfinity
```

```
{4193.8, 3754.43, 3179.21, 2509.36, 1817.75, 1222.32, 3521.07, 2972.37,
 2306.89, 1555.06, 822.556, 239.908, 3625.32, 2902.15, 2077.78, 1228.81, 469.109}
```

```
1 / GamATot111 * t0ToFemtoSecond
```

```
41.6827
```

## Decay matrix with exclusively radiative decay widths

```
matRad:=SparseArray[{
(* No core holes *)
{idxconfig["216"],idxconfig["216"]}→-GamRTot216,{idxconfig["225"],idxconfig["216"]}→GamR225v216,
{idxconfig["215"],idxconfig["215"]}→-GamRTot215,{idxconfig["224"],idxconfig["215"]}→GamR224v215,
{idxconfig["206"],idxconfig["206"]}→-GamRTot206,{idxconfig["215"],idxconfig["206"]}→GamR215v206,
{idxconfig["214"],idxconfig["214"]}→-GamRTot214,{idxconfig["223"],idxconfig["214"]}→GamR223v214,
{idxconfig["205"],idxconfig["205"]}→-GamRTot205,{idxconfig["214"],idxconfig["205"]}→GamR214v205,
{idxconfig["213"],idxconfig["213"]}→-GamRTot213,{idxconfig["222"],idxconfig["213"]}→GamR222v213,
{idxconfig["204"],idxconfig["204"]}→-GamRTot204,{idxconfig["213"],idxconfig["204"]}→GamR213v204,
{idxconfig["212"],idxconfig["212"]}→-GamRTot212,{idxconfig["221"],idxconfig["212"]}→GamR221v212,
{idxconfig["203"],idxconfig["203"]}→-GamRTot203,{idxconfig["212"],idxconfig["203"]}→GamR212v203,
{idxconfig["211"],idxconfig["211"]}→-GamRTot211,{idxconfig["220"],idxconfig["211"]}→GamR220v211,
{idxconfig["202"],idxconfig["202"]}→-GamRTot202,{idxconfig["211"],idxconfig["202"]}→GamR211v202,
{idxconfig["201"],idxconfig["201"]}→-GamRTot201,{idxconfig["210"],idxconfig["201"]}→GamR210v201,

(* Single core holes *)
{idxconfig["110"],idxconfig["110"]}→-GamRTot110,{idxconfig["200"],idxconfig["110"]}→GamR200v110,
{idxconfig["101"],idxconfig["101"]}→-GamRTot101,{idxconfig["200"],idxconfig["101"]}→GamR200v101,
{idxconfig["110"],idxconfig["101"]}→GamR110v101,

(* Double core holes *)
{idxconfig["010"],idxconfig["010"]}→-GamRTot010,{idxconfig["100"],idxconfig["010"]}→GamR100v010,
{idxconfig["001"],idxconfig["001"]}→-GamRTot001,{idxconfig["100"],idxconfig["001"]}→GamR100v001,
{idxconfig["010"],idxconfig["001"]}→GamR010v001},
{Length[configurations],Length[configurations]}]
```

```
Chop[Transpose[Eigenvectors[matRad]].DiagonalMatrix[Eigenvalues[matRad]].
    Inverse[Transpose[Eigenvectors[matRad]]] - matRad] == SparseArray[{},
{Length[configurations], Length[configurations]}]
```

```
True
```

## Probabilities at infinite time

```
eigval = Eigenvalues[matRad]
```

$\{-0.000151332, -0.0000563657, -4.87891\times10^{-7}, -4.62189\times10^{-7}, -3.90745\times10^{-7}, -3.56251\times10^{-7}, -2.7969\times10^{-7}, -2.39355\times10^{-7}, -1.7363\times10^{-7}, -1.34533\times10^{-7}, -8.72344\times10^{-8}, -5.75167\times10^{-8}, -2.89245\times10^{-8}, -1.4163\times10^{-8}, -6.0715\times10^{-13}, -1.8002\times10^{-13}, 0., 0., 0., 0., 0., 0., 0., 0., 0., 0., 0., 0., 0., 0., 0., 0., 0., 0., 0., 0., 0., 0., 0., 0., 0., 0., 0., 0., 0., 0., 0., 0., 0., 0., 0., 0., 0., 0., 0., 0., 0., 0., 0., 0., 0., 0., 0., 0., 0., 0., 0., 0., 0.\}$

```
diagelem = Map[DiscreteDelta, eigval]
```

```
{0, 0, 0, 0, 0, 0, 0, 0, 0, 0, 0, 0, 0, 0, 0, 0, 1, 1, 1, 1, 1, 1, 1, 1, 1, 1, 1, 1, 1,
 1, 1, 1, 1, 1, 1, 1, 1, 1, 1, 1, 1, 1, 1, 1, 1, 1, 1, 1, 1, 1, 1, 1, 1, 1, 1, 1, 1, 1, 1, 1, 1, 1, 1, 1, 1, 1}
```

```
expGamInf = Transpose[Eigenvectors[matRad]].DiagonalMatrix[diagelem].Inverse[Transpose[Eigenvectors[matRad]]];
```

## Integral over the probabilities

$$\text{diagelemintexp}[t\_] := \text{Table}\left[\text{If}\left[\text{eigval}[[i]] \neq 0, \frac{e^{\text{eigval}[[i]]\,(t-\text{posinfinity})} - 1}{\text{eigval}[[i]]}, t - \text{posinfinity}\right], \{i, 1, \text{Length}[\text{eigval}]\}\right]$$

$$\text{diagelemint}[t\_] := \text{Table}\left[\text{If}\left[\text{eigval}[[i]] \neq 0, \frac{-1}{\text{eigval}[[i]]}, t - \text{posinfinity}\right], \{i, 1, \text{Length}[\text{eigval}]\}\right]$$

```
diagelemintexp[10 000 * posinfinity] - diagelemint[10 000 * posinfinity]
```

```
{0., 0., 0., 0., 0., 0., 0., 0., 0., 0., 0., 0., 0., 0., -1.64291×10^12, -5.55081×10^12,
 0., 0., 0., 0., 0., 0., 0., 0., 0., 0., 0., 0., 0., 0., 0., 0., 0., 0., 0., 0., 0., 0., 0.,
 0., 0., 0., 0., 0., 0., 0., 0., 0., 0., 0., 0., 0., 0., 0., 0., 0., 0., 0., 0., 0., 0., 0., 0.}
```

```
diagelemintexp[1*^9 * posinfinity] - diagelemint[1*^9 * posinfinity]
```

```
{0., 0., 0., 0., 0., 0., 0., 0., 0., 0., 0., 0., 0., 0., 0., 0., 0., 0., 0., 0., 0., 0., 0., 0., 0., 0., 0., 0., 0., 0., 0., 0.,
 0., 0., 0., 0., 0., 0., 0., 0., 0., 0., 0., 0., 0., 0., 0., 0., 0., 0., 0., 0., 0., 0., 0., 0., 0., 0., 0., 0., 0., 0., 0.}
```

```
posinfinityrad := 1*^10 * posinfinity
```

```
expIntGam =
  Transpose[Eigenvectors[matRad]].DiagonalMatrix[diagelemint[posinfinityrad]].Inverse[Transpose[Eigenvectors[matRad]]];
```

# Crater integration of fluorescence

Quantities to be determined over the crater:

```
probability[sol_]:=expGamInf.(Values[sol[[1]]]/.t->posinfinity)
```

```
probabilityaction[sol_] :=
 NIntegrate[Values[sol[[1]]], {t, neginfinity, posinfinity}, AccuracyGoal → 10, MaxRecursion → 20, Method → "LocalAdaptive"] +
  expIntGam.(Values[sol[[1]]] /. t -> posinfinity)
```

Compute fluorescence for a fraction of the peak x-ray fluences on the beam axis:

```
fluorescenceprofile[pulseenergy_,photonenergy_,tauX_,nintsteps_,nint_]:=Module[{J0Xpeak,J0Xcur,sol,jxcrater},
J0Xpeak=2*Sqrt[Log[2]/Pi]/tauX*peakfluence[pulseenergy,photonenergy];
J0Xcur=J0Xpeak/nintsteps*nint;
jxcrater[t_]:=jxgaussian[J0Xcur,tauX,t];
sol=solveRateEquations[photonenergy,jxcrater,neginfinity,posinfinity,1/10000];
Join[{J0Xcur},probability[sol],probabilityaction[sol]]
]
```

```
tabfluorescenceprof[pulseenergy_,photonenergy_,tauX_,nintsteps_]:=Module[{nint},
Table[fluorescenceprofile[pulseenergy,photonenergy,tauX,nintsteps,nint],
{nint,nintsteps,0,-1}]
]
```

Create interpolation functions for all charge states:

```
interpolfluorescence[tabdata_]:=Module[{nint},
Table[
ListInterpolation[tabdata[[All,nint]],{tabdata[[All,1]]}],
{nint,2,Length[tabdata[[1]]]}]
]
```

Evaluate all fluorescence at a specific spatial point:

```
fluorescenceint[funyields_,pulseenergy_,photonenergy_,tauX_,rx_,ry_]:=Module[{jj0x,nint},
jj0x=J0Xfun[pulseenergy,photonenergy,tauX,rx,ry];
Table[funyields[[nint]][jj0x],{nint,1,Length[funyields]}]
]
```

Integration of the fluorescence of the beam area. The integral needs to be normalized to the integration area:

```
fluorescencebeam[funyields_, pulseenergy_, photonenergy_, tauX_] :=
 1/(Pi * (40 * MicrometerToBohr)^2) * NIntegrate[fluorescenceint[funyields, pulseenergy, photonenergy, tauX, rx, 0] * 2 * Pi * rx,
   {rx, 0, 40 * MicrometerToBohr}, MaxRecursion → 20, Method → "LocalAdaptive", AccuracyGoal → 10]
```

Probability and probability action over the crater:

```
fluorescencecrateranalysis[pulseenergy_,photoenergy_,pulseduration_,nint_]:=Module[{tabionyi,funionyi},
tabionyi=tabfluorescenceprof[pulseenergy,photoenergy,pulseduration,nint];
funionyi=interpolfluorescence[tabionyi];
fluorescencebeam[funionyi,pulseenergy,photoenergy,pulseduration]
]
```

Calculation of the photon yields for x-ray radiative transitions greater 800 eV:

```
photonyields[pulseenergy_] :=
 Module[{crava, probaction, fluorescence, xraySpectrumFluorescence, xraySpectrumFluorescenceNorm},
  crava = fluorescencecrateranalysis[pulseenergy, omegaX, tauX, nintdata];
(* First Length[configurations] elements are the probability.
   Second Length[configurations] elements are the probability action *)
probaction = crava[[Length[configurations] + 1 ;; 2 * Length[configurations]]];
fluorescence = fluorecencematrix.probaction;
xraySpectrumFluorescence = Table[If[fluorecenceenergy[[i]] * HartreeToeV >= 800,
     {fluorecenceenergy[[i]] * HartreeToeV, fluorescence[[i]]}, {0, 0}], {i, 1, Length[fluorescence]}];
xraySpectrumFluorescenceNorm = Table[{xraySpectrumFluorescence[[i, 1]], 1/Total[xraySpectrumFluorescence[[ ;; , 2]]] *
       xraySpectrumFluorescence[[i, 2]]}, {i, 1, Length[xraySpectrumFluorescence]}];
  xraySpectrumFluorescenceNorm
 ]
```

# Fluorescence spectrum from the plain rate equations

## FWHM diameter of the LCLS beam: 5 μm

FWHM of the crater profile:

```
rhoXx := 5 * MicrometerToBohr
rhoYy := rhoXx
```

```
xraySpectrumFluorescenceNorm = photonyields[pulseenergy];
```

```
ListPlot[xraySpectrumFluorescenceNorm, PlotRange → {{835, 900}, {0, 1}}, Filling → Bottom,
 FillingStyle → Thick, PlotMarkers → {Automatic, Small}, PlotStyle → {Red, Thick}, AxesLabel → {"ωX [eV]", "y(ωX)"},
 LabelStyle → {FontFamily → "Helvetica", FontSize → 14}, AxesStyle → Arrowheads[Automatic]]
```

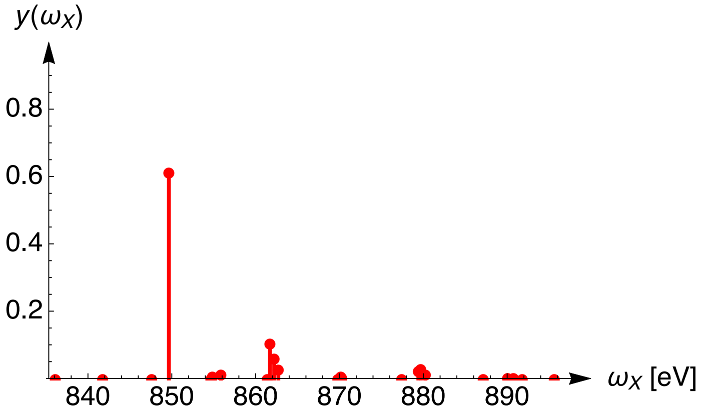


```
spectrumFluorescenceStates = Table[
   {i, fluorescencetransitions[[i]], fluorecenceenergy[[i]] * HartreeToeV, xraySpectrumFluorescenceNorm[[i, 2]]}, {i, 1, 100}];
```

```
Sort[spectrumFluorescenceStates, #1[[4]] > #2[[4]] &][[1 ;; 20]] // TableForm
```

| | | | | | | | | | |
|---|---|---|---|---|---|---|---|---|---|
| 2 | 1s(1) | 2s(2) | 2p(6) | ⟶ | 1s(2) | 2s(2) | 2p(5) | 849.65 | 0.613206 |
| 15 | 1s(1) | 2s(2) | 2p(4) | ⟶ | 1s(2) | 2s(2) | 2p(3) | 861.711 | 0.105255 |
| 17 | 1s(1) | 2s(1) | 2p(5) | ⟶ | 1s(2) | 2s(1) | 2p(4) | 862.214 | 0.061057 |
| 47 | 1s(1) | 2s(1) | 2p(3) | ⟶ | 1s(2) | 2s(1) | 2p(2) | 879.7 | 0.0297709 |
| 90 | 1s(1) | 2s(0) | 2p(1) | ⟶ | 1s(2) | 2s(0) | 2p(0) | 915.795 | 0.0277772 |
| 20 | 1s(1) | 2s(0) | 2p(6) | ⟶ | 1s(2) | 2s(0) | 2p(5) | 862.711 | 0.0277679 |
| 80 | 1s(1) | 2s(0) | 2p(2) | ⟶ | 1s(2) | 2s(0) | 2p(1) | 902.212 | 0.0235667 |
| 50 | 1s(1) | 2s(0) | 2p(4) | ⟶ | 1s(2) | 2s(0) | 2p(3) | 879.407 | 0.023564 |
| 77 | 1s(1) | 2s(1) | 2p(1) | ⟶ | 1s(2) | 2s(1) | 2p(0) | 903.298 | 0.0159406 |
| 45 | 1s(1) | 2s(2) | 2p(2) | ⟶ | 1s(2) | 2s(2) | 2p(1) | 880.245 | 0.0135248 |
| 8 | 1s(1) | 2s(1) | 2p(6) | ⟶ | 1s(2) | 2s(1) | 2p(5) | 855.868 | 0.0132096 |
| 89 | 1s(1) | 2s(1) | 2p(0) | ⟶ | 1s(2) | 2s(0) | 2p(0) | 906.634 | 0.0121974 |
| 6 | 1s(1) | 2s(2) | 2p(5) | ⟶ | 1s(2) | 2s(2) | 2p(4) | 854.849 | 0.00707937 |
| 31 | 1s(1) | 2s(1) | 2p(4) | ⟶ | 1s(2) | 2s(1) | 2p(3) | 870.171 | 0.00703977 |
| 11 | 1s(0) | 2s(2) | 2p(6) | ⟶ | 1s(1) | 2s(2) | 2p(5) | 946.736 | 0.00420832 |
| 63 | 1s(1) | 2s(1) | 2p(2) | ⟶ | 1s(2) | 2s(1) | 2p(1) | 890.758 | 0.003039 |
| 66 | 1s(1) | 2s(0) | 2p(3) | ⟶ | 1s(2) | 2s(0) | 2p(2) | 890.066 | 0.00284203 |
| 34 | 1s(1) | 2s(0) | 2p(5) | ⟶ | 1s(2) | 2s(0) | 2p(4) | 870.276 | 0.00273772 |
| 29 | 1s(1) | 2s(2) | 2p(3) | ⟶ | 1s(2) | 2s(2) | 2p(2) | 870.192 | 0.00205931 |
| 36 | 1s(0) | 2s(2) | 2p(4) | ⟶ | 1s(1) | 2s(2) | 2p(3) | 962.102 | 0.00095704 |

## FWHM diameter of the LCLS beam: 7.3 μm

FWHM of the crater profile:

```
rhoXx := 7.3 * MicrometerToBohr
rhoYy := rhoXx
```

```
xraySpectrumFluorescenceNorm = photonyields[pulseenergy];
```

```
ListPlot[xraySpectrumFluorescenceNorm, PlotRange → {{835, 900}, {0, 1}}, Filling → Bottom,
 FillingStyle → Thick, PlotMarkers → {Automatic, Small}, PlotStyle → {Red, Thick}, AxesLabel → {"ωX [eV]", "y(ωX)"},
 LabelStyle → {FontFamily → "Helvetica", FontSize → 14}, AxesStyle → Arrowheads[Automatic]]
```

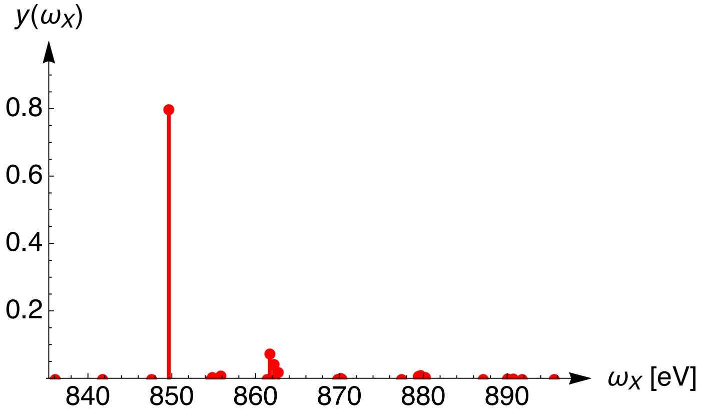


```
spectrumFluorescenceStates = Table[
   {i, fluorescencetransitions[[i]], fluorecenceenergy[[i]] * HartreeToeV, xraySpectrumFluorescenceNorm[[i, 2]]}, {i, 1, 100}];
```

```
Sort[spectrumFluorescenceStates, #1[[4]] > #2[[4]] &][[1 ;; 20]] // TableForm
```

| | | | | | | | | | |
|---|---|---|---|---|---|---|---|---|---|
| 2 | 1s(1) | 2s(2) | 2p(6) | ⟶ 1s(2) | 2s(2) | 2p(5) | 849.65 | 0.800496 |
| 15 | 1s(1) | 2s(2) | 2p(4) | ⟶ 1s(2) | 2s(2) | 2p(3) | 861.711 | 0.0750594 |
| 17 | 1s(1) | 2s(1) | 2p(5) | ⟶ 1s(2) | 2s(1) | 2p(4) | 862.214 | 0.0441727 |
| 20 | 1s(1) | 2s(0) | 2p(6) | ⟶ 1s(2) | 2s(0) | 2p(5) | 862.711 | 0.020525 |
| 47 | 1s(1) | 2s(1) | 2p(3) | ⟶ 1s(2) | 2s(1) | 2p(2) | 879.7 | 0.0109324 |
| 8 | 1s(1) | 2s(1) | 2p(6) | ⟶ 1s(2) | 2s(1) | 2p(5) | 855.868 | 0.00985875 |
| 50 | 1s(1) | 2s(0) | 2p(4) | ⟶ 1s(2) | 2s(0) | 2p(3) | 879.407 | 0.00871511 |
| 6 | 1s(1) | 2s(2) | 2p(5) | ⟶ 1s(2) | 2s(2) | 2p(4) | 854.849 | 0.00513209 |
| 45 | 1s(1) | 2s(2) | 2p(2) | ⟶ 1s(2) | 2s(2) | 2p(1) | 880.245 | 0.00499291 |
| 80 | 1s(1) | 2s(0) | 2p(2) | ⟶ 1s(2) | 2s(0) | 2p(1) | 902.212 | 0.00421657 |
| 77 | 1s(1) | 2s(1) | 2p(1) | ⟶ 1s(2) | 2s(1) | 2p(0) | 903.298 | 0.00289981 |
| 11 | 1s(0) | 2s(2) | 2p(6) | ⟶ 1s(1) | 2s(2) | 2p(5) | 946.736 | 0.00283562 |
| 31 | 1s(1) | 2s(1) | 2p(4) | ⟶ 1s(2) | 2s(1) | 2p(3) | 870.171 | 0.0026339 |
| 90 | 1s(1) | 2s(0) | 2p(1) | ⟶ 1s(2) | 2s(0) | 2p(0) | 915.795 | 0.00242016 |
| 89 | 1s(1) | 2s(1) | 2p(0) | ⟶ 1s(2) | 2s(0) | 2p(0) | 906.634 | 0.00110106 |
| 34 | 1s(1) | 2s(0) | 2p(5) | ⟶ 1s(2) | 2s(0) | 2p(4) | 870.276 | 0.00104491 |
| 29 | 1s(1) | 2s(2) | 2p(3) | ⟶ 1s(2) | 2s(2) | 2p(2) | 870.192 | 0.000760569 |
| 63 | 1s(1) | 2s(1) | 2p(2) | ⟶ 1s(2) | 2s(1) | 2p(1) | 890.758 | 0.000558182 |
| 66 | 1s(1) | 2s(0) | 2p(3) | ⟶ 1s(2) | 2s(0) | 2p(2) | 890.066 | 0.000520652 |
| 36 | 1s(0) | 2s(2) | 2p(4) | ⟶ 1s(1) | 2s(2) | 2p(3) | 962.102 | 0.000327188 |

## FWHM diameter of the LCLS beam: 8 μm

FWHM of the crater profile:

```
rhoXx := 8 * MicrometerToBohr
rhoYy := rhoXx
```

```
xraySpectrumFluorescenceNorm = photonyields[pulseenergy];
```

```
ListPlot[xraySpectrumFluorescenceNorm, PlotRange → {{835, 900}, {0, 1}}, Filling → Bottom,
 FillingStyle → Thick, PlotMarkers → {Automatic, Small}, PlotStyle → {Red, Thick}, AxesLabel → {"ωX [eV]", "y(ωX)"},
 LabelStyle → {FontFamily → "Helvetica", FontSize → 14}, AxesStyle → Arrowheads[Automatic]]
```

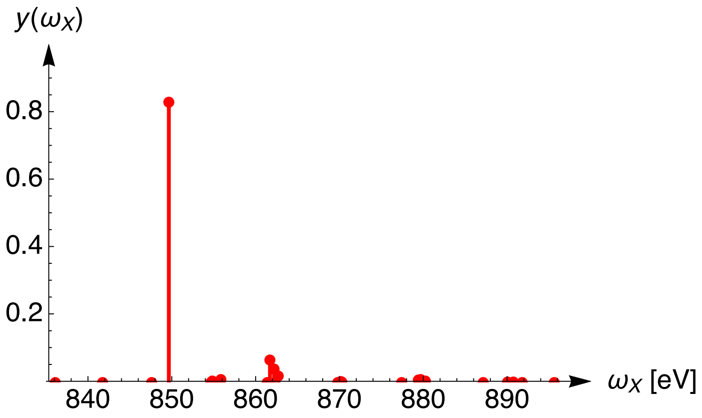


```
spectrumFluorescenceStates = Table[
   {i, fluorescencetransitions[[i]], fluorecenceenergy[[i]] * HartreeToeV, xraySpectrumFluorescenceNorm[[i, 2]]}, {i, 1, 100}];
```

```
Sort[spectrumFluorescenceStates, #1[[4]] > #2[[4]] &][[1 ;; 20]] // TableForm
```

| | | | |
|---|---|---|---|
| 2 | 1s(1) 2s(2) 2p(6) ⟶ 1s(2) 2s(2) 2p(5) | 849.65 | 0.830958 |
| 15 | 1s(1) 2s(2) 2p(4) ⟶ 1s(2) 2s(2) 2p(3) | 861.711 | 0.0663562 |
| 17 | 1s(1) 2s(1) 2p(5) ⟶ 1s(2) 2s(1) 2p(4) | 862.214 | 0.0391442 |
| 20 | 1s(1) 2s(0) 2p(6) ⟶ 1s(2) 2s(0) 2p(5) | 862.711 | 0.0182555 |
| 8 | 1s(1) 2s(1) 2p(6) ⟶ 1s(2) 2s(1) 2p(5) | 855.868 | 0.00878416 |
| 47 | 1s(1) 2s(1) 2p(3) ⟶ 1s(2) 2s(1) 2p(2) | 879.7 | 0.00815247 |
| 50 | 1s(1) 2s(0) 2p(4) ⟶ 1s(2) 2s(0) 2p(3) | 879.407 | 0.00650701 |
| 6 | 1s(1) 2s(2) 2p(5) ⟶ 1s(2) 2s(2) 2p(4) | 854.849 | 0.00454981 |
| 45 | 1s(1) 2s(2) 2p(2) ⟶ 1s(2) 2s(2) 2p(1) | 880.245 | 0.00372652 |
| 80 | 1s(1) 2s(0) 2p(2) ⟶ 1s(2) 2s(0) 2p(1) | 902.212 | 0.00263101 |
| 11 | 1s(0) 2s(2) 2p(6) ⟶ 1s(1) 2s(2) 2p(5) | 946.736 | 0.00248541 |
| 31 | 1s(1) 2s(1) 2p(4) ⟶ 1s(2) 2s(1) 2p(3) | 870.171 | 0.00197041 |
| 77 | 1s(1) 2s(1) 2p(1) ⟶ 1s(2) 2s(1) 2p(0) | 903.298 | 0.00181391 |
| 90 | 1s(1) 2s(0) 2p(1) ⟶ 1s(2) 2s(0) 2p(0) | 915.795 | 0.00126387 |
| 34 | 1s(1) 2s(0) 2p(5) ⟶ 1s(2) 2s(0) 2p(4) | 870.276 | 0.000784188 |
| 89 | 1s(1) 2s(1) 2p(0) ⟶ 1s(2) 2s(0) 2p(0) | 906.634 | 0.000578114 |
| 29 | 1s(1) 2s(2) 2p(3) ⟶ 1s(2) 2s(2) 2p(2) | 870.192 | 0.000567749 |
| 63 | 1s(1) 2s(1) 2p(2) ⟶ 1s(2) 2s(1) 2p(1) | 890.758 | 0.000349691 |
| 66 | 1s(1) 2s(0) 2p(3) ⟶ 1s(2) 2s(0) 2p(2) | 890.066 | 0.000326078 |
| 36 | 1s(0) 2s(2) 2p(4) ⟶ 1s(1) 2s(2) 2p(3) | 962.102 | 0.000241408 |

## FWHM diameter of the LCLS beam: 10 μm

FWHM of the crater profile:

```
rhoXx := 10 * MicrometerToBohr
rhoYy := rhoXx
```

```
xraySpectrumFluorescenceNorm = photonyields[pulseenergy];
```

```
ListPlot[xraySpectrumFluorescenceNorm, PlotRange → {{835, 900}, {0, 1}}, Filling → Bottom,
 FillingStyle → Thick, PlotMarkers → {Automatic, Small}, PlotStyle → {Red, Thick}, AxesLabel → {"ωX [eV]", "y(ωX)"},
 LabelStyle → {FontFamily → "Helvetica", FontSize → 14}, AxesStyle → Arrowheads[Automatic]]
```

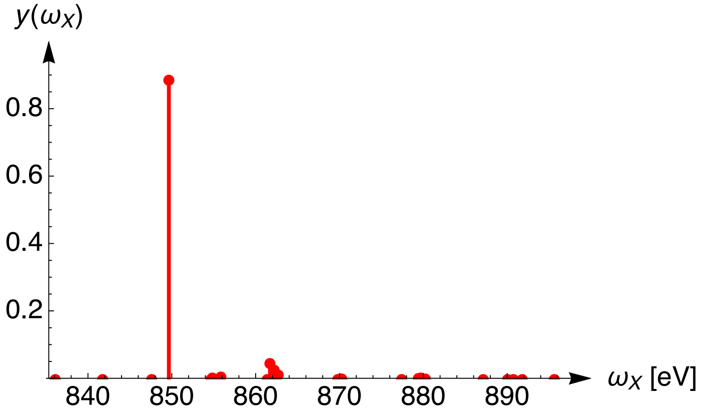


```
spectrumFluorescenceStates = Table[
   {i, fluorescencetransitions[[i]], fluorecenceenergy[[i]] * HartreeToeV, xraySpectrumFluorescenceNorm[[i, 2]]}, {i, 1, 100}];
```

```
Sort[spectrumFluorescenceStates, #1[[4]] > #2[[4]] &][[1 ;; 20]] // TableForm
```

| | | | | |
|---|---|---|---|---|
| 2 | 1s(1) 2s(2) 2p(6) ⟶ 1s(2) 2s(2) 2p(5) | | 849.65 | 0.887905 |
| 15 | 1s(1) 2s(2) 2p(4) ⟶ 1s(2) 2s(2) 2p(3) | | 861.711 | 0.0472392 |
| 17 | 1s(1) 2s(1) 2p(5) ⟶ 1s(2) 2s(1) 2p(4) | | 862.214 | 0.0279909 |
| 20 | 1s(1) 2s(0) 2p(6) ⟶ 1s(2) 2s(0) 2p(5) | | 862.711 | 0.0131448 |
| 8 | 1s(1) 2s(1) 2p(6) ⟶ 1s(2) 2s(1) 2p(5) | | 855.868 | 0.00634657 |
| 47 | 1s(1) 2s(1) 2p(3) ⟶ 1s(2) 2s(1) 2p(2) | | 879.7 | 0.00379933 |
| 6 | 1s(1) 2s(2) 2p(5) ⟶ 1s(2) 2s(2) 2p(4) | | 854.849 | 0.00325624 |
| 50 | 1s(1) 2s(0) 2p(4) ⟶ 1s(2) 2s(0) 2p(3) | | 879.407 | 0.00303955 |
| 11 | 1s(0) 2s(2) 2p(6) ⟶ 1s(1) 2s(2) 2p(5) | | 946.736 | 0.00174233 |
| 45 | 1s(1) 2s(2) 2p(2) ⟶ 1s(2) 2s(2) 2p(1) | | 880.245 | 0.00173946 |
| 31 | 1s(1) 2s(1) 2p(4) ⟶ 1s(2) 2s(1) 2p(3) | | 870.171 | 0.000923797 |
| 80 | 1s(1) 2s(0) 2p(2) ⟶ 1s(2) 2s(0) 2p(1) | | 902.212 | 0.00079125 |
| 77 | 1s(1) 2s(1) 2p(1) ⟶ 1s(2) 2s(1) 2p(0) | | 903.298 | 0.000547969 |
| 34 | 1s(1) 2s(0) 2p(5) ⟶ 1s(2) 2s(0) 2p(4) | | 870.276 | 0.000369809 |
| 29 | 1s(1) 2s(2) 2p(3) ⟶ 1s(2) 2s(2) 2p(2) | | 870.192 | 0.000265105 |
| 90 | 1s(1) 2s(0) 2p(1) ⟶ 1s(2) 2s(0) 2p(0) | | 915.795 | 0.000245453 |
| 89 | 1s(1) 2s(1) 2p(0) ⟶ 1s(2) 2s(0) 2p(0) | | 906.634 | 0.000113375 |
| 36 | 1s(0) 2s(2) 2p(4) ⟶ 1s(1) 2s(2) 2p(3) | | 962.102 | 0.000110383 |
| 63 | 1s(1) 2s(1) 2p(2) ⟶ 1s(2) 2s(1) 2p(1) | | 890.758 | 0.000105937 |
| 66 | 1s(1) 2s(0) 2p(3) ⟶ 1s(2) 2s(0) 2p(2) | | 890.066 | 0.0000987332 |

## FWHM diameter of the LCLS beam: 12 μm

FWHM of the crater profile:

```
rhoXx := 12 * MicrometerToBohr
rhoYy := rhoXx
```

```
xraySpectrumFluorescenceNorm = photonyields[pulseenergy];
```

```
ListPlot[xraySpectrumFluorescenceNorm, PlotRange → {{835, 900}, {0, 1}}, Filling → Bottom,
 FillingStyle → Thick, PlotMarkers → {Automatic, Small}, PlotStyle → {Red, Thick}, AxesLabel → {"ωX [eV]", "y(ωX)"},
 LabelStyle → {FontFamily → "Helvetica", FontSize → 14}, AxesStyle → Arrowheads[Automatic]]
```

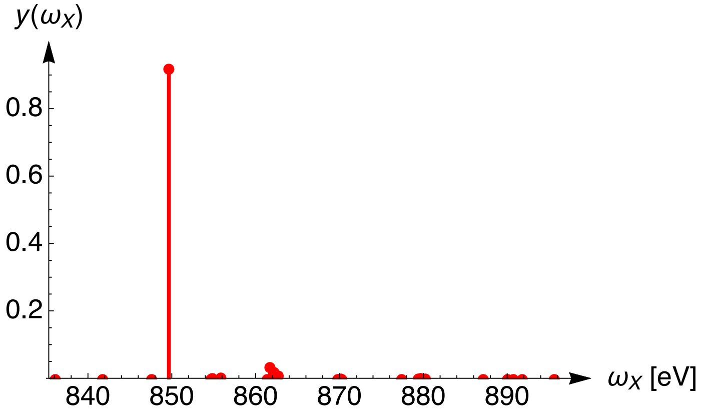


```
spectrumFluorescenceStates = Table[
   {i, fluorescencetransitions[[i]], fluorecenceenergy[[i]] * HartreeToeV, xraySpectrumFluorescenceNorm[[i, 2]]}, {i, 1, 100}];
```

```
Sort[spectrumFluorescenceStates, #1[[4]] > #2[[4]] &][[1 ;; 20]] // TableForm
```

| | | | | |
|---|---|---|---|---|
| 2 | 1s(1) 2s(2) 2p(6) ⟶ 1s(2) 2s(2) 2p(5) | 849.65 | 0.920432 |
| 15 | 1s(1) 2s(2) 2p(4) ⟶ 1s(2) 2s(2) 2p(3) | 861.711 | 0.0347519 |
| 17 | 1s(1) 2s(1) 2p(5) ⟶ 1s(2) 2s(1) 2p(4) | 862.214 | 0.0206432 |
| 20 | 1s(1) 2s(0) 2p(6) ⟶ 1s(2) 2s(0) 2p(5) | 862.711 | 0.00973267 |
| 8 | 1s(1) 2s(1) 2p(6) ⟶ 1s(2) 2s(1) 2p(5) | 855.868 | 0.00470845 |
| 6 | 1s(1) 2s(2) 2p(5) ⟶ 1s(2) 2s(2) 2p(4) | 854.849 | 0.00240272 |
| 47 | 1s(1) 2s(1) 2p(3) ⟶ 1s(2) 2s(1) 2p(2) | 879.7 | 0.00196426 |
| 50 | 1s(1) 2s(0) 2p(4) ⟶ 1s(2) 2s(0) 2p(3) | 879.407 | 0.00157354 |
| 11 | 1s(0) 2s(2) 2p(6) ⟶ 1s(1) 2s(2) 2p(5) | 946.736 | 0.00127115 |
| 45 | 1s(1) 2s(2) 2p(2) ⟶ 1s(2) 2s(2) 2p(1) | 880.245 | 0.000900111 |
| 31 | 1s(1) 2s(1) 2p(4) ⟶ 1s(2) 2s(1) 2p(3) | 870.171 | 0.000479236 |
| 80 | 1s(1) 2s(0) 2p(2) ⟶ 1s(2) 2s(0) 2p(1) | 902.212 | 0.000285287 |
| 77 | 1s(1) 2s(1) 2p(1) ⟶ 1s(2) 2s(1) 2p(0) | 903.298 | 0.000198055 |
| 34 | 1s(1) 2s(0) 2p(5) ⟶ 1s(2) 2s(0) 2p(4) | 870.276 | 0.000192468 |
| 29 | 1s(1) 2s(2) 2p(3) ⟶ 1s(2) 2s(2) 2p(2) | 870.192 | 0.000137213 |
| 90 | 1s(1) 2s(0) 2p(1) ⟶ 1s(2) 2s(0) 2p(0) | 915.795 | 0.0000617491 |
| 36 | 1s(0) 2s(2) 2p(4) ⟶ 1s(1) 2s(2) 2p(3) | 962.102 | 0.0000564822 |
| 38 | 1s(0) 2s(1) 2p(5) ⟶ 1s(1) 2s(1) 2p(4) | 961.709 | 0.0000484579 |
| 63 | 1s(1) 2s(1) 2p(2) ⟶ 1s(2) 2s(1) 2p(1) | 890.758 | 0.0000383493 |
| 66 | 1s(1) 2s(0) 2p(3) ⟶ 1s(2) 2s(0) 2p(2) | 890.066 | 0.0000357328 |

## FWHM diameter of the LCLS beam: 15 μm

FWHM of the crater profile:

```
rhoXx := 15 * MicrometerToBohr
rhoYy := rhoXx
```

```
xraySpectrumFluorescenceNorm = photonyields[pulseenergy];
```

```
ListPlot[xraySpectrumFluorescenceNorm, PlotRange → {{835, 900}, {0, 1}}, Filling → Bottom,
 FillingStyle → Thick, PlotMarkers → {Automatic, Small}, PlotStyle → {Red, Thick}, AxesLabel → {"ωX [eV]", "y(ωX)"},
 LabelStyle → {FontFamily → "Helvetica", FontSize → 14}, AxesStyle → Arrowheads[Automatic]]
```

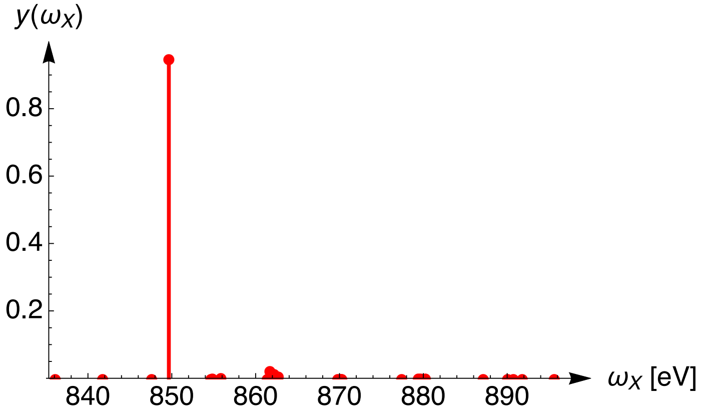


```
spectrumFluorescenceStates = Table[
   {i, fluorescencetransitions[[i]], fluorecenceenergy[[i]] * HartreeToeV, xraySpectrumFluorescenceNorm[[i, 2]]}, {i, 1, 100}];
```

```
Sort[spectrumFluorescenceStates, #1[[4]] > #2[[4]] &][[1 ;; 20]] // TableForm
```

| | | | | |
|---|---|---|---|---|
| 2 | 1s(1) 2s(2) 2p(6) | ⟶ 1s(2) 2s(2) 2p(5) | 849.65 | 0.948077 |
| 15 | 1s(1) 2s(2) 2p(4) | ⟶ 1s(2) 2s(2) 2p(3) | 861.711 | 0.0233166 |
| 17 | 1s(1) 2s(1) 2p(5) | ⟶ 1s(2) 2s(1) 2p(4) | 862.214 | 0.0138795 |
| 20 | 1s(1) 2s(0) 2p(6) | ⟶ 1s(2) 2s(0) 2p(5) | 862.711 | 0.00656559 |
| 8 | 1s(1) 2s(1) 2p(6) | ⟶ 1s(2) 2s(1) 2p(5) | 855.868 | 0.00318167 |
| 6 | 1s(1) 2s(2) 2p(5) | ⟶ 1s(2) 2s(2) 2p(4) | 854.849 | 0.0016162 |
| 47 | 1s(1) 2s(1) 2p(3) | ⟶ 1s(2) 2s(1) 2p(2) | 879.7 | 0.000851566 |
| 11 | 1s(0) 2s(2) 2p(6) | ⟶ 1s(1) 2s(2) 2p(5) | 946.736 | 0.000847077 |
| 50 | 1s(1) 2s(0) 2p(4) | ⟶ 1s(2) 2s(0) 2p(3) | 879.407 | 0.000682941 |
| 45 | 1s(1) 2s(2) 2p(2) | ⟶ 1s(2) 2s(2) 2p(1) | 880.245 | 0.000390516 |
| 31 | 1s(1) 2s(1) 2p(4) | ⟶ 1s(2) 2s(1) 2p(3) | 870.171 | 0.00020836 |
| 34 | 1s(1) 2s(0) 2p(5) | ⟶ 1s(2) 2s(0) 2p(4) | 870.276 | 0.0000839061 |
| 80 | 1s(1) 2s(0) 2p(2) | ⟶ 1s(2) 2s(0) 2p(1) | 902.212 | 0.0000794199 |
| 29 | 1s(1) 2s(2) 2p(3) | ⟶ 1s(2) 2s(2) 2p(2) | 870.192 | 0.0000595422 |
| 77 | 1s(1) 2s(1) 2p(1) | ⟶ 1s(2) 2s(1) 2p(0) | 903.298 | 0.0000552472 |
| 36 | 1s(0) 2s(2) 2p(4) | ⟶ 1s(1) 2s(2) 2p(3) | 962.102 | 0.0000242811 |
| 38 | 1s(0) 2s(1) 2p(5) | ⟶ 1s(1) 2s(1) 2p(4) | 961.709 | 0.0000208752 |
| 90 | 1s(1) 2s(0) 2p(1) | ⟶ 1s(2) 2s(0) 2p(0) | 915.795 | 0.0000110435 |
| 63 | 1s(1) 2s(1) 2p(2) | ⟶ 1s(2) 2s(1) 2p(1) | 890.758 | 0.0000107112 |
| 66 | 1s(1) 2s(0) 2p(3) | ⟶ 1s(2) 2s(0) 2p(2) | 890.066 | $9.97853 \times 10^{-6}$ |

## FWHM diameter of the LCLS beam: 18 μm

FWHM of the crater profile:

```
rhoXx := 18 * MicrometerToBohr
rhoYy := rhoXx

xraySpectrumFluorescenceNorm = photonyields[pulseenergy];
```

```
ListPlot[xraySpectrumFluorescenceNorm, PlotRange → {{835, 900}, {0, 1}}, Filling → Bottom,
 FillingStyle → Thick, PlotMarkers → {Automatic, Small}, PlotStyle → {Red, Thick}, AxesLabel → {"ωX [eV]", "y(ωX)"},
 LabelStyle → {FontFamily → "Helvetica", FontSize → 14}, AxesStyle → Arrowheads[Automatic]]
```

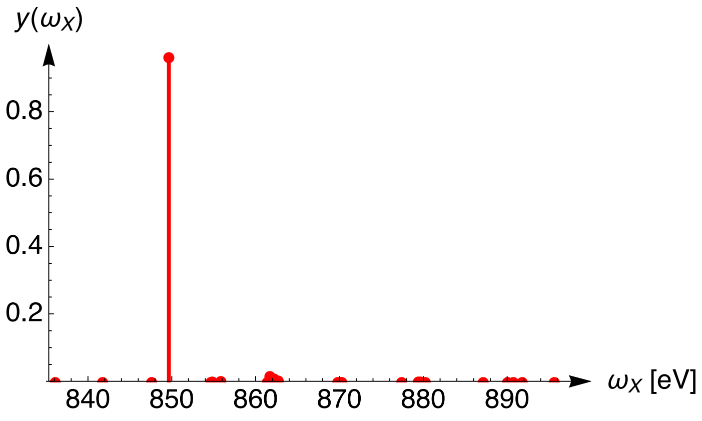


```
spectrumFluorescenceStates = Table[
   {i, fluorescencetransitions[[i]], fluorecenceenergy[[i]] * HartreeToeV, xraySpectrumFluorescenceNorm[[i, 2]]}, {i, 1, 100}];
```

```
Sort[spectrumFluorescenceStates, #1[[4]] > #2[[4]] &][[1 ;; 20]] // TableForm
```

| | | | | |
|---|---|---|---|---|
| 2 | 1s(1) 2s(2) 2p(6) ⟶ 1s(2) 2s(2) 2p(5) | 849.65 | 0.963539 |
| 15 | 1s(1) 2s(2) 2p(4) ⟶ 1s(2) 2s(2) 2p(3) | 861.711 | 0.0166137 |
| 17 | 1s(1) 2s(1) 2p(5) ⟶ 1s(2) 2s(1) 2p(4) | 862.214 | 0.00990089 |
| 20 | 1s(1) 2s(0) 2p(6) ⟶ 1s(2) 2s(0) 2p(5) | 862.711 | 0.00469221 |
| 8 | 1s(1) 2s(1) 2p(6) ⟶ 1s(2) 2s(1) 2p(5) | 855.868 | 0.00227598 |
| 6 | 1s(1) 2s(2) 2p(5) ⟶ 1s(2) 2s(2) 2p(4) | 854.849 | 0.00115321 |
| 11 | 1s(0) 2s(2) 2p(6) ⟶ 1s(1) 2s(2) 2p(5) | 946.736 | 0.000601374 |
| 47 | 1s(1) 2s(1) 2p(3) ⟶ 1s(2) 2s(1) 2p(2) | 879.7 | 0.000423524 |
| 50 | 1s(1) 2s(0) 2p(4) ⟶ 1s(2) 2s(0) 2p(3) | 879.407 | 0.00033987 |
| 45 | 1s(1) 2s(2) 2p(2) ⟶ 1s(2) 2s(2) 2p(1) | 880.245 | 0.000194302 |
| 31 | 1s(1) 2s(1) 2p(4) ⟶ 1s(2) 2s(1) 2p(3) | 870.171 | 0.000103792 |
| 34 | 1s(1) 2s(0) 2p(5) ⟶ 1s(2) 2s(0) 2p(4) | 870.276 | 0.0000418586 |
| 29 | 1s(1) 2s(2) 2p(3) ⟶ 1s(2) 2s(2) 2p(2) | 870.192 | 0.0000296287 |
| 80 | 1s(1) 2s(0) 2p(2) ⟶ 1s(2) 2s(0) 2p(1) | 902.212 | 0.0000274783 |
| 77 | 1s(1) 2s(1) 2p(1) ⟶ 1s(2) 2s(1) 2p(0) | 903.298 | 0.0000191362 |
| 36 | 1s(0) 2s(2) 2p(4) ⟶ 1s(1) 2s(2) 2p(3) | 962.102 | 0.0000120211 |
| 38 | 1s(0) 2s(1) 2p(5) ⟶ 1s(1) 2s(1) 2p(4) | 961.709 | 0.0000103467 |
| 41 | 1s(0) 2s(0) 2p(6) ⟶ 1s(1) 2s(0) 2p(5) | 961.84 | $4.74091 \times 10^{-6}$ |
| 63 | 1s(1) 2s(1) 2p(2) ⟶ 1s(2) 2s(1) 2p(1) | 890.758 | $3.71262 \times 10^{-6}$ |
| 66 | 1s(1) 2s(0) 2p(3) ⟶ 1s(2) 2s(0) 2p(2) | 890.066 | $3.45834 \times 10^{-6}$ |

## FWHM diameter of the LCLS beam: 20 μm

FWHM of the crater profile:

```
rhoXx := 20 * MicrometerToBohr
rhoYy := rhoXx

xraySpectrumFluorescenceNorm = photonyields[pulseenergy];
```

```
ListPlot[xraySpectrumFluorescenceNorm, PlotRange → {{835, 900}, {0, 1}}, Filling → Bottom,
 FillingStyle → Thick, PlotMarkers → {Automatic, Small}, PlotStyle → {Red, Thick}, AxesLabel → {"ωX [eV]", "y(ωX)"},
 LabelStyle → {FontFamily → "Helvetica", FontSize → 14}, AxesStyle → Arrowheads[Automatic]]
```

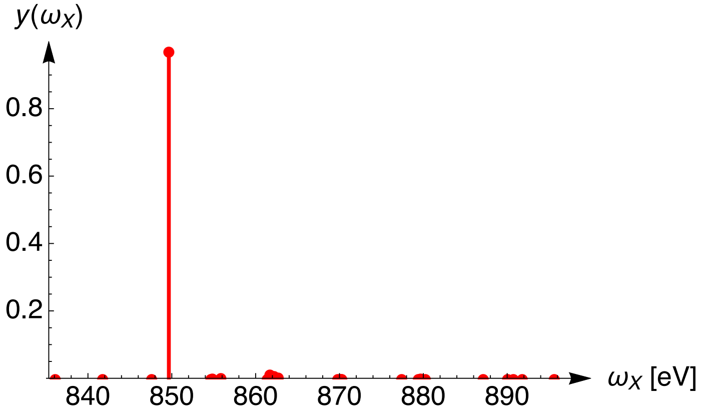


```
spectrumFluorescenceStates = Table[
   {i, fluorescencetransitions[[i]], fluorecenceenergy[[i]] * HartreeToeV, xraySpectrumFluorescenceNorm[[i, 2]]}, {i, 1, 100}];
```

```
Sort[spectrumFluorescenceStates, #1[[4]] > #2[[4]] &][[1 ;; 20]] // TableForm
```

| | | | | | | | | | |
|---|---|---|---|---|---|---|---|---|---|
| 2 | 1s(1) | 2s(2) | 2p(6) | ⟶ | 1s(2) | 2s(2) | 2p(5) | 849.65 | 0.97032 |
| 15 | 1s(1) | 2s(2) | 2p(4) | ⟶ | 1s(2) | 2s(2) | 2p(3) | 861.711 | 0.0136077 |
| 17 | 1s(1) | 2s(1) | 2p(5) | ⟶ | 1s(2) | 2s(1) | 2p(4) | 862.214 | 0.00811356 |
| 20 | 1s(1) | 2s(0) | 2p(6) | ⟶ | 1s(2) | 2s(0) | 2p(5) | 862.711 | 0.00384825 |
| 8 | 1s(1) | 2s(1) | 2p(6) | ⟶ | 1s(2) | 2s(1) | 2p(5) | 855.868 | 0.00186739 |
| 6 | 1s(1) | 2s(2) | 2p(5) | ⟶ | 1s(2) | 2s(2) | 2p(4) | 854.849 | 0.000945132 |
| 11 | 1s(0) | 2s(2) | 2p(6) | ⟶ | 1s(1) | 2s(2) | 2p(5) | 946.736 | 0.000491834 |
| 47 | 1s(1) | 2s(1) | 2p(3) | ⟶ | 1s(2) | 2s(1) | 2p(2) | 879.7 | 0.000281601 |
| 50 | 1s(1) | 2s(0) | 2p(4) | ⟶ | 1s(2) | 2s(0) | 2p(3) | 879.407 | 0.000226041 |
| 45 | 1s(1) | 2s(2) | 2p(2) | ⟶ | 1s(2) | 2s(2) | 2p(1) | 880.245 | 0.000129214 |
| 31 | 1s(1) | 2s(1) | 2p(4) | ⟶ | 1s(2) | 2s(1) | 2p(3) | 870.171 | 0.0000690593 |
| 34 | 1s(1) | 2s(0) | 2p(5) | ⟶ | 1s(2) | 2s(0) | 2p(4) | 870.276 | 0.0000278689 |
| 29 | 1s(1) | 2s(2) | 2p(3) | ⟶ | 1s(2) | 2s(2) | 2p(2) | 870.192 | 0.0000197046 |
| 80 | 1s(1) | 2s(0) | 2p(2) | ⟶ | 1s(2) | 2s(0) | 2p(1) | 902.212 | 0.0000148101 |
| 77 | 1s(1) | 2s(1) | 2p(1) | ⟶ | 1s(2) | 2s(1) | 2p(0) | 903.298 | 0.0000103195 |
| 36 | 1s(0) | 2s(2) | 2p(4) | ⟶ | 1s(1) | 2s(2) | 2p(3) | 962.102 | $7.97705 \times 10^{-6}$ |
| 38 | 1s(0) | 2s(1) | 2p(5) | ⟶ | 1s(1) | 2s(1) | 2p(4) | 961.709 | $6.86938 \times 10^{-6}$ |
| 41 | 1s(0) | 2s(0) | 2p(6) | ⟶ | 1s(1) | 2s(0) | 2p(5) | 961.84 | $3.15026 \times 10^{-6}$ |
| 63 | 1s(1) | 2s(1) | 2p(2) | ⟶ | 1s(2) | 2s(1) | 2p(1) | 890.758 | $2.00256 \times 10^{-6}$ |
| 66 | 1s(1) | 2s(0) | 2p(3) | ⟶ | 1s(2) | 2s(0) | 2p(2) | 890.066 | $1.86532 \times 10^{-6}$ |

# Modified rate equations

```
Solve[a / (1 - a) == shake, a]
```

$$\left\{\left\{a \to \frac{\text{shake}}{1+\text{shake}}\right\}\right\}$$

Photoionization shake off from Table I of Ref. [3]:

$$\text{valshakeoff} := \frac{0.16}{1+0.16}$$

Photoionization shake off from Table III of Ref. [3]:

$$\text{coreshakeoff} := \frac{0.23}{1+0.23}$$

Double Auger decay partial probabilities from Table I of Ref. [2]:

```
p2pm3 := 2.5 / 100
p2sm12pm2 := 2.9 / 100
p2sm22pm1 := 0.5 / 100
pNem3 := p2pm3 + p2sm12pm2 + p2sm22pm1
```

Probabilities from Table I of Ref. [4]:

```
daNe2p := 0.9267
daNe3p := 0.0597
```

```
d = daNe3p / (daNe2p + daNe3p)
```

```
0.0605231
```

```
1 - d
```

```
0.939477
```

Double Auger decay fractions:

```
da223v126 = p2pm3 / pNem3 * d
```

```
0.0256454
```

```
da214v126 = p2sm12pm2 / pNem3 * d
```

```
0.0297486
```

```
da205v126 = p2sm22pm1 / pNem3 * d
```

```
0.00512908
```

```
daTot126 := da223v126 + da214v126 + da205v126
```

## Multiple photoionization of the valence electrons

```
req225[en_, jx_] := P225'[t] ==
  (1 - valshakeoff) * xsc225v226[en] * jx[t] * P226[t] - xscTot225[en] * jx[t] * P225[t] + GamR225v216 * P216[t] + GamR225v126 * P126[t]

req216[en_, jx_] := P216'[t] ==
  (1 - valshakeoff) * xsc216v226[en] * jx[t] * P226[t] - xscTot216[en] * jx[t] * P216[t] + GamR216v126 * P126[t] - GamRTot216 * P216[t]
```

## Multiple photoionization of core and valence electrons

```
req126[en_, jx_] := P126'[t] ==
  (1 - coreshakeoff) * xsc126v226[en] * jx[t] * P226[t] - xscTot126[en] * jx[t] * P126[t] - GamATot126 * P126[t] - GamRTot126 * P126[t]

req125[en_, jx_] :=
 P125'[t] == coreshakeoff * xsc126v226[en] * jx[t] * P226[t] + xsc125v225[en] * jx[t] * P225[t] + xsc125v126[en] * jx[t] * P126[t] -
   xscTot125[en] * jx[t] * P125[t] - GamATot125 * P125[t] + GamR125v116 * P116[t] + GamR125v026 * P026[t] - GamRTot125 * P125[t]
```

## Double Auger decay

```
req224[en_, jx_] := P224'[t] == valshakeoff * xsc225v226[en] * jx[t] * P226[t] + xsc224v225[en] * jx[t] * P225[t] -
   xscTot224[en] * jx[t] * P224[t] + (1 - daTot126) * GamA224v126 * P126[t] + GamR224v215 * P215[t] + GamR224v125 * P125[t]

req215[en_, jx_] := P215'[t] == valshakeoff * xsc216v226[en] * jx[t] * P226[t] + xsc215v225[en] * jx[t] * P225[t] +
   xsc215v216[en] * jx[t] * P216[t] - xscTot215[en] * jx[t] * P215[t] + (1 - daTot126) * GamA215v126 * P126[t] +
   GamR215v206 * P206[t] + GamR215v125 * P125[t] + GamR215v116 * P116[t] - GamRTot215 * P215[t]

req206[en_, jx_] := P206'[t] == xsc206v216[en] * jx[t] * P216[t] -
   xscTot206[en] * jx[t] * P206[t] + (1 - daTot126) * GamA206v126 * P126[t] + GamR206v116 * P116[t] - GamRTot206 * P206[t]

req223[en_, jx_] := P223'[t] == xsc223v224[en] * jx[t] * P224[t] - xscTot223[en] * jx[t] * P223[t] +
   da223v126 * GamATot126 * P126[t] + GamA223v125 * P125[t] + GamR223v214 * P214[t] + GamR223v124 * P124[t]
```

```
req214[en_, jx_] := P214'[t] == xsc214v224[en] * jx[t] * P224[t] + xsc214v215[en] * jx[t] * P215[t] -
    xscTot214[en] * jx[t] * P214[t] + da214v126 * GamATot126 * P126[t] + GamA214v125 * P125[t] + GamA214v116 * P116[t] +
    GamR214v205 * P205[t] + GamR214v124 * P124[t] + GamR214v115 * P115[t] - GamRTot214 * P214[t]

req205[en_, jx_] := P205'[t] == xsc205v215[en] * jx[t] * P215[t] +
    xsc205v206[en] * jx[t] * P206[t] - xscTot205[en] * jx[t] * P205[t] + da205v126 * GamATot126 * P126[t] +
    GamA205v125 * P125[t] + GamA205v116 * P116[t] + GamR205v115 * P115[t] + GamR205v106 * P106[t] - GamRTot205 * P205[t]
```

# Fluorescence spectrum from the modified rate equations

## FWHM diameter of the LCLS beam: 5 μm

FWHM of the crater profile:

```
rhoXx := 5 * MicrometerToBohr
rhoYy := rhoXx

xraySpectrumFluorescenceNorm = photonyields[pulseenergy];
```

```
ListPlot[xraySpectrumFluorescenceNorm, PlotRange → {{835, 900}, {0, 1}}, Filling → Bottom,
 FillingStyle → Thick, PlotMarkers → {Automatic, Small}, PlotStyle → {Red, Thick}, AxesLabel → {"ωX [eV]", "y(ωX)"},
 LabelStyle → {FontFamily → "Helvetica", FontSize → 14}, AxesStyle → Arrowheads[Automatic]]
```

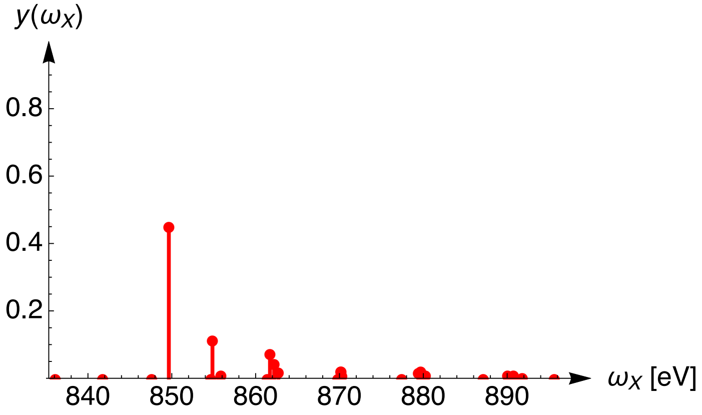


```
spectrumFluorescenceStates = Table[
   {i, fluorescencetransitions[[i]], fluorecenceenergy[[i]] * HartreeToeV, xraySpectrumFluorescenceNorm[[i, 2]]}, {i, 1, 100}];
```

```
Sort[spectrumFluorescenceStates, #1[[4]] > #2[[4]] &][[1 ;; 20]] // TableForm
```

| | | | | |
|---|---|---|---|---|
| 2 | 1s(1) 2s(2) 2p(6) ⟶ 1s(2) 2s(2) 2p(5) | 849.65 | 0.450812 |
| 6 | 1s(1) 2s(2) 2p(5) ⟶ 1s(2) 2s(2) 2p(4) | 854.849 | 0.11351 |
| 90 | 1s(1) 2s(0) 2p(1) ⟶ 1s(2) 2s(0) 2p(0) | 915.795 | 0.0891262 |
| 15 | 1s(1) 2s(2) 2p(4) ⟶ 1s(2) 2s(2) 2p(3) | 861.711 | 0.0738328 |
| 17 | 1s(1) 2s(1) 2p(5) ⟶ 1s(2) 2s(1) 2p(4) | 862.214 | 0.0438985 |
| 89 | 1s(1) 2s(1) 2p(0) ⟶ 1s(2) 2s(0) 2p(0) | 906.634 | 0.0411325 |
| 47 | 1s(1) 2s(1) 2p(3) ⟶ 1s(2) 2s(1) 2p(2) | 879.7 | 0.0219116 |
| 29 | 1s(1) 2s(2) 2p(3) ⟶ 1s(2) 2s(2) 2p(2) | 870.192 | 0.0212033 |
| 31 | 1s(1) 2s(1) 2p(4) ⟶ 1s(2) 2s(1) 2p(3) | 870.171 | 0.0210671 |
| 20 | 1s(1) 2s(0) 2p(6) ⟶ 1s(2) 2s(0) 2p(5) | 862.711 | 0.0192131 |
| 80 | 1s(1) 2s(0) 2p(2) ⟶ 1s(2) 2s(0) 2p(1) | 902.212 | 0.0173907 |
| 50 | 1s(1) 2s(0) 2p(4) ⟶ 1s(2) 2s(0) 2p(3) | 879.407 | 0.0168725 |
| 77 | 1s(1) 2s(1) 2p(1) ⟶ 1s(2) 2s(1) 2p(0) | 903.298 | 0.0119941 |
| 63 | 1s(1) 2s(1) 2p(2) ⟶ 1s(2) 2s(1) 2p(1) | 890.758 | 0.0104098 |
| 8 | 1s(1) 2s(1) 2p(6) ⟶ 1s(2) 2s(1) 2p(5) | 855.868 | 0.010275 |
| 45 | 1s(1) 2s(2) 2p(2) ⟶ 1s(2) 2s(2) 2p(1) | 880.245 | 0.00967105 |
| 66 | 1s(1) 2s(0) 2p(3) ⟶ 1s(2) 2s(0) 2p(2) | 890.066 | 0.00945346 |
| 34 | 1s(1) 2s(0) 2p(5) ⟶ 1s(2) 2s(0) 2p(4) | 870.276 | 0.00894237 |
| 11 | 1s(0) 2s(2) 2p(6) ⟶ 1s(1) 2s(2) 2p(5) | 946.736 | 0.00309367 |
| 61 | 1s(1) 2s(2) 2p(1) ⟶ 1s(2) 2s(2) 2p(0) | 891.819 | 0.00181767 |

## FWHM diameter of the LCLS beam: 7.3 μm

FWHM of the crater profile:

```
rhoXx := 7.3 * MicrometerToBohr
rhoYy := rhoXx

xraySpectrumFluorescenceNorm = photonyields[pulseenergy];
```

```
ListPlot[xraySpectrumFluorescenceNorm, PlotRange → {{835, 900}, {0, 1}}, Filling → Bottom,
 FillingStyle → Thick, PlotMarkers → {Automatic, Small}, PlotStyle → {Red, Thick}, AxesLabel → {"ωX [eV]", "y(ωX)"},
 LabelStyle → {FontFamily → "Helvetica", FontSize → 14}, AxesStyle → Arrowheads[Automatic]]
```

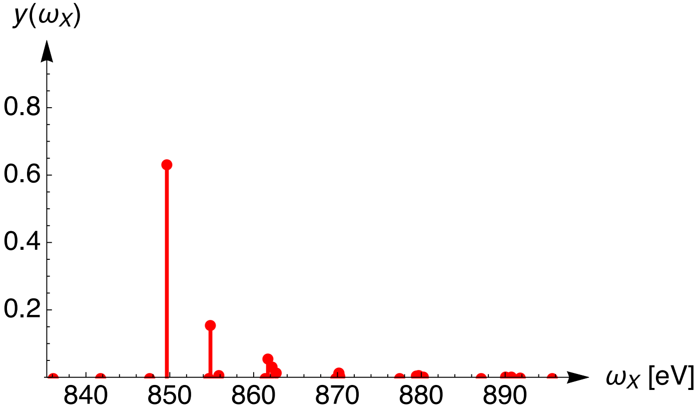


```
spectrumFluorescenceStates = Table[
   {i, fluorescencetransitions[[i]], fluorecenceenergy[[i]] * HartreeToeV, xraySpectrumFluorescenceNorm[[i, 2]]}, {i, 1, 100}];
```

```
Sort[spectrumFluorescenceStates, #1[[4]] > #2[[4]] &][[1 ;; 20]] // TableForm
```

| | | | | |
|---|---|---|---|---|
| 2 | 1s(1) 2s(2) 2p(6) ⟶ 1s(2) 2s(2) 2p(5) | 849.65 | 0.634414 |
| 6 | 1s(1) 2s(2) 2p(5) ⟶ 1s(2) 2s(2) 2p(4) | 854.849 | 0.156323 |
| 15 | 1s(1) 2s(2) 2p(4) ⟶ 1s(2) 2s(2) 2p(3) | 861.711 | 0.0567516 |
| 17 | 1s(1) 2s(1) 2p(5) ⟶ 1s(2) 2s(1) 2p(4) | 862.214 | 0.0342244 |
| 29 | 1s(1) 2s(2) 2p(3) ⟶ 1s(2) 2s(2) 2p(2) | 870.192 | 0.0156689 |
| 20 | 1s(1) 2s(0) 2p(6) ⟶ 1s(2) 2s(0) 2p(5) | 862.711 | 0.0153027 |
| 90 | 1s(1) 2s(0) 2p(1) ⟶ 1s(2) 2s(0) 2p(0) | 915.795 | 0.0150348 |
| 31 | 1s(1) 2s(1) 2p(4) ⟶ 1s(2) 2s(1) 2p(3) | 870.171 | 0.0141869 |
| 47 | 1s(1) 2s(1) 2p(3) ⟶ 1s(2) 2s(1) 2p(2) | 879.7 | 0.00866891 |
| 8 | 1s(1) 2s(1) 2p(6) ⟶ 1s(2) 2s(1) 2p(5) | 855.868 | 0.00826839 |
| 89 | 1s(1) 2s(1) 2p(0) ⟶ 1s(2) 2s(0) 2p(0) | 906.634 | 0.00725958 |
| 50 | 1s(1) 2s(0) 2p(4) ⟶ 1s(2) 2s(0) 2p(3) | 879.407 | 0.00672092 |
| 34 | 1s(1) 2s(0) 2p(5) ⟶ 1s(2) 2s(0) 2p(4) | 870.276 | 0.00619189 |
| 45 | 1s(1) 2s(2) 2p(2) ⟶ 1s(2) 2s(2) 2p(1) | 880.245 | 0.00384794 |
| 63 | 1s(1) 2s(1) 2p(2) ⟶ 1s(2) 2s(1) 2p(1) | 890.758 | 0.00363392 |
| 80 | 1s(1) 2s(0) 2p(2) ⟶ 1s(2) 2s(0) 2p(1) | 902.212 | 0.00335031 |
| 66 | 1s(1) 2s(0) 2p(3) ⟶ 1s(2) 2s(0) 2p(2) | 890.066 | 0.00327228 |
| 77 | 1s(1) 2s(1) 2p(1) ⟶ 1s(2) 2s(1) 2p(0) | 903.298 | 0.00235063 |
| 11 | 1s(0) 2s(2) 2p(6) ⟶ 1s(1) 2s(2) 2p(5) | 946.736 | 0.00224698 |
| 61 | 1s(1) 2s(2) 2p(1) ⟶ 1s(2) 2s(2) 2p(0) | 891.819 | 0.000693455 |

## FWHM diameter of the LCLS beam: 8 μm

FWHM of the crater profile:

```
rhoXx := 8 * MicrometerToBohr
rhoYy := rhoXx
```

```
xraySpectrumFluorescenceNorm = photonyields[pulseenergy];
```

```
ListPlot[xraySpectrumFluorescenceNorm, PlotRange → {{835, 900}, {0, 1}}, Filling → Bottom,
 FillingStyle → Thick, PlotMarkers → {Automatic, Small}, PlotStyle → {Red, Thick}, AxesLabel → {"ωX [eV]", "y(ωX)"},
 LabelStyle → {FontFamily → "Helvetica", FontSize → 14}, AxesStyle → Arrowheads[Automatic]]
```

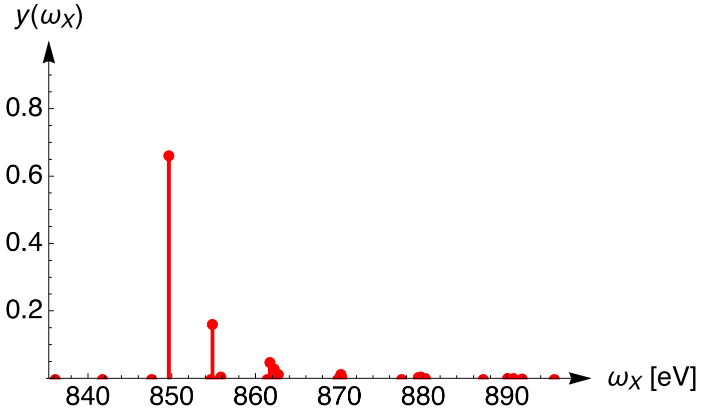


```
spectrumFluorescenceStates = Table[
   {i, fluorescencetransitions[[i]], fluorecenceenergy[[i]] * HartreeToeV, xraySpectrumFluorescenceNorm[[i, 2]]}, {i, 1, 100}];
```

```
Sort[spectrumFluorescenceStates, #1[[4]] > #2[[4]] &][[1 ;; 20]] // TableForm
```

| | | | | |
|---|---|---|---|---|
| 2 | 1s(1) 2s(2) 2p(6) ⟶ 1s(2) 2s(2) 2p(5) | 849.65 | 0.662998 |
| 6 | 1s(1) 2s(2) 2p(5) ⟶ 1s(2) 2s(2) 2p(4) | 854.849 | 0.162716 |
| 15 | 1s(1) 2s(2) 2p(4) ⟶ 1s(2) 2s(2) 2p(3) | 861.711 | 0.0505087 |
| 17 | 1s(1) 2s(1) 2p(5) ⟶ 1s(2) 2s(1) 2p(4) | 862.214 | 0.0305312 |
| 29 | 1s(1) 2s(2) 2p(3) ⟶ 1s(2) 2s(2) 2p(2) | 870.192 | 0.0138513 |
| 20 | 1s(1) 2s(0) 2p(6) ⟶ 1s(2) 2s(0) 2p(5) | 862.711 | 0.0137014 |
| 31 | 1s(1) 2s(1) 2p(4) ⟶ 1s(2) 2s(1) 2p(3) | 870.171 | 0.0123226 |
| 90 | 1s(1) 2s(0) 2p(1) ⟶ 1s(2) 2s(0) 2p(0) | 915.795 | 0.00923475 |
| 8 | 1s(1) 2s(1) 2p(6) ⟶ 1s(2) 2s(1) 2p(5) | 855.868 | 0.00741705 |
| 47 | 1s(1) 2s(1) 2p(3) ⟶ 1s(2) 2s(1) 2p(2) | 879.7 | 0.00650756 |
| 34 | 1s(1) 2s(0) 2p(5) ⟶ 1s(2) 2s(0) 2p(4) | 870.276 | 0.00540473 |
| 50 | 1s(1) 2s(0) 2p(4) ⟶ 1s(2) 2s(0) 2p(3) | 879.407 | 0.00505117 |
| 89 | 1s(1) 2s(1) 2p(0) ⟶ 1s(2) 2s(0) 2p(0) | 906.634 | 0.00449129 |
| 45 | 1s(1) 2s(2) 2p(2) ⟶ 1s(2) 2s(2) 2p(1) | 880.245 | 0.00289123 |
| 63 | 1s(1) 2s(1) 2p(2) ⟶ 1s(2) 2s(1) 2p(1) | 890.758 | 0.00266957 |
| 66 | 1s(1) 2s(0) 2p(3) ⟶ 1s(2) 2s(0) 2p(2) | 890.066 | 0.00240054 |
| 80 | 1s(1) 2s(0) 2p(2) ⟶ 1s(2) 2s(0) 2p(1) | 902.212 | 0.0021042 |
| 11 | 1s(0) 2s(2) 2p(6) ⟶ 1s(1) 2s(2) 2p(5) | 946.736 | 0.00198261 |
| 77 | 1s(1) 2s(1) 2p(1) ⟶ 1s(2) 2s(1) 2p(0) | 903.298 | 0.00148017 |
| 61 | 1s(1) 2s(2) 2p(1) ⟶ 1s(2) 2s(2) 2p(0) | 891.819 | 0.000517443 |

## FWHM diameter of the LCLS beam: 10 μm

FWHM of the crater profile:

```
rhoXx := 10 * MicrometerToBohr
rhoYy := rhoXx

xraySpectrumFluorescenceNorm = photonyields[pulseenergy];
```

```
ListPlot[xraySpectrumFluorescenceNorm, PlotRange → {{835, 900}, {0, 1}}, Filling → Bottom,
 FillingStyle → Thick, PlotMarkers → {Automatic, Small}, PlotStyle → {Red, Thick}, AxesLabel → {"ωX [eV]", "y(ωX)"},
 LabelStyle → {FontFamily → "Helvetica", FontSize → 14}, AxesStyle → Arrowheads[Automatic]]
```

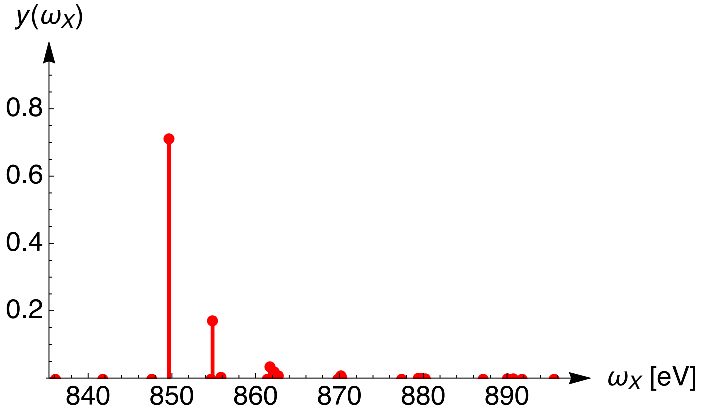


```
spectrumFluorescenceStates = Table[
   {i, fluorescencetransitions[[i]], fluorecenceenergy[[i]] * HartreeToeV, xraySpectrumFluorescenceNorm[[i, 2]]}, {i, 1, 100}];
```

```
Sort[spectrumFluorescenceStates, #1[[4]] > #2[[4]] &][[1 ;; 20]] // TableForm
```

| | | | | |
|---|---|---|---|---|
| 2 | 1s(1) 2s(2) 2p(6) ⟶ 1s(2) 2s(2) 2p(5) | 849.65 | 0.714075 |
| 6 | 1s(1) 2s(2) 2p(5) ⟶ 1s(2) 2s(2) 2p(4) | 854.849 | 0.1739 |
| 15 | 1s(1) 2s(2) 2p(4) ⟶ 1s(2) 2s(2) 2p(3) | 861.711 | 0.0362424 |
| 17 | 1s(1) 2s(1) 2p(5) ⟶ 1s(2) 2s(1) 2p(4) | 862.214 | 0.0220036 |
| 20 | 1s(1) 2s(0) 2p(6) ⟶ 1s(2) 2s(0) 2p(5) | 862.711 | 0.00994281 |
| 29 | 1s(1) 2s(2) 2p(3) ⟶ 1s(2) 2s(2) 2p(2) | 870.192 | 0.00981306 |
| 31 | 1s(1) 2s(1) 2p(4) ⟶ 1s(2) 2s(1) 2p(3) | 870.171 | 0.00843247 |
| 8 | 1s(1) 2s(1) 2p(6) ⟶ 1s(2) 2s(1) 2p(5) | 855.868 | 0.00540179 |
| 34 | 1s(1) 2s(0) 2p(5) ⟶ 1s(2) 2s(0) 2p(4) | 870.276 | 0.00373361 |
| 47 | 1s(1) 2s(1) 2p(3) ⟶ 1s(2) 2s(1) 2p(2) | 879.7 | 0.00305639 |
| 90 | 1s(1) 2s(0) 2p(1) ⟶ 1s(2) 2s(0) 2p(0) | 915.795 | 0.00268373 |
| 50 | 1s(1) 2s(0) 2p(4) ⟶ 1s(2) 2s(0) 2p(3) | 879.407 | 0.00237764 |
| 11 | 1s(0) 2s(2) 2p(6) ⟶ 1s(1) 2s(2) 2p(5) | 946.736 | 0.00140044 |
| 45 | 1s(1) 2s(2) 2p(2) ⟶ 1s(2) 2s(2) 2p(1) | 880.245 | 0.00136024 |
| 89 | 1s(1) 2s(1) 2p(0) ⟶ 1s(2) 2s(0) 2p(0) | 906.634 | 0.00132271 |
| 63 | 1s(1) 2s(1) 2p(2) ⟶ 1s(2) 2s(1) 2p(1) | 890.758 | 0.00120339 |
| 66 | 1s(1) 2s(0) 2p(3) ⟶ 1s(2) 2s(0) 2p(2) | 890.066 | 0.00107927 |
| 80 | 1s(1) 2s(0) 2p(2) ⟶ 1s(2) 2s(0) 2p(1) | 902.212 | 0.000637647 |
| 77 | 1s(1) 2s(1) 2p(1) ⟶ 1s(2) 2s(1) 2p(0) | 903.298 | 0.000450645 |
| 22 | 1s(0) 2s(2) 2p(5) ⟶ 1s(1) 2s(2) 2p(4) | 953.636 | 0.000313098 |

## FWHM diameter of the LCLS beam: 12 μm

FWHM of the crater profile:

```
rhoXx := 12 * MicrometerToBohr
rhoYy := rhoXx
```

```
xraySpectrumFluorescenceNorm = photonyields[pulseenergy];
```

```
ListPlot[xraySpectrumFluorescenceNorm, PlotRange → {{835, 900}, {0, 1}}, Filling → Bottom,
 FillingStyle → Thick, PlotMarkers → {Automatic, Small}, PlotStyle → {Red, Thick}, AxesLabel → {"ωX [eV]", "y(ωX)"},
 LabelStyle → {FontFamily → "Helvetica", FontSize → 14}, AxesStyle → Arrowheads[Automatic]]
```

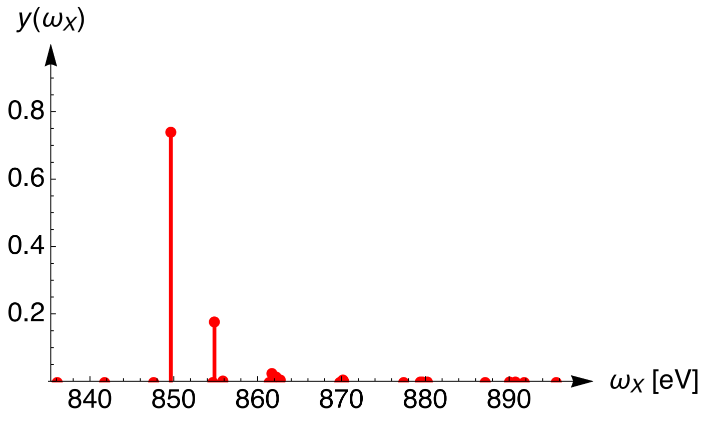


```
spectrumFluorescenceStates = Table[
   {i, fluorescencetransitions[[i]], fluorecenceenergy[[i]] * HartreeToeV, xraySpectrumFluorescenceNorm[[i, 2]]}, {i, 1, 100}];
```

```
Sort[spectrumFluorescenceStates, #1[[4]] > #2[[4]] &][[1 ;; 20]] // TableForm
```

```
2    1s(1) 2s(2) 2p(6) ⟶ 1s(2) 2s(2) 2p(5)   849.65    0.741842
6    1s(1) 2s(2) 2p(5) ⟶ 1s(2) 2s(2) 2p(4)   854.849   0.179841
15   1s(1) 2s(2) 2p(4) ⟶ 1s(2) 2s(2) 2p(3)   861.711   0.0267194
17   1s(1) 2s(1) 2p(5) ⟶ 1s(2) 2s(1) 2p(4)   862.214   0.0162619
20   1s(1) 2s(0) 2p(6) ⟶ 1s(2) 2s(0) 2p(5)   862.711   0.00737724
29   1s(1) 2s(2) 2p(3) ⟶ 1s(2) 2s(2) 2p(2)   870.192   0.00718209
31   1s(1) 2s(1) 2p(4) ⟶ 1s(2) 2s(1) 2p(3)   870.171   0.00604496
8    1s(1) 2s(1) 2p(6) ⟶ 1s(2) 2s(1) 2p(5)   855.868   0.00401635
34   1s(1) 2s(0) 2p(5) ⟶ 1s(2) 2s(0) 2p(4)   870.276   0.00269131
47   1s(1) 2s(1) 2p(3) ⟶ 1s(2) 2s(1) 2p(2)   879.7     0.00158345
50   1s(1) 2s(0) 2p(4) ⟶ 1s(2) 2s(0) 2p(3)   879.407   0.00123336
11   1s(0) 2s(2) 2p(6) ⟶ 1s(1) 2s(2) 2p(5)   946.736   0.00102377
90   1s(1) 2s(0) 2p(1) ⟶ 1s(2) 2s(0) 2p(0)   915.795   0.000946726
45   1s(1) 2s(2) 2p(2) ⟶ 1s(2) 2s(2) 2p(1)   880.245   0.000705383
63   1s(1) 2s(1) 2p(2) ⟶ 1s(2) 2s(1) 2p(1)   890.758   0.000608893
66   1s(1) 2s(0) 2p(3) ⟶ 1s(2) 2s(0) 2p(2)   890.066   0.000545264
89   1s(1) 2s(1) 2p(0) ⟶ 1s(2) 2s(0) 2p(0)   906.634   0.000470083
80   1s(1) 2s(0) 2p(2) ⟶ 1s(2) 2s(0) 2p(1)   902.212   0.000230365
22   1s(0) 2s(2) 2p(5) ⟶ 1s(1) 2s(2) 2p(4)   953.636   0.000227387
77   1s(1) 2s(1) 2p(1) ⟶ 1s(2) 2s(1) 2p(0)   903.298   0.000163228
```

## FWHM diameter of the LCLS beam: 15 μm

FWHM of the crater profile:

```
rhoXx := 15 * MicrometerToBohr
rhoYy := rhoXx
```

```
xraySpectrumFluorescenceNorm = photonyields[pulseenergy];
```

```
ListPlot[xraySpectrumFluorescenceNorm, PlotRange → {{835, 900}, {0, 1}}, Filling → Bottom,
 FillingStyle → Thick, PlotMarkers → {Automatic, Small}, PlotStyle → {Red, Thick}, AxesLabel → {"ωX [eV]", "y(ωX)"},
 LabelStyle → {FontFamily → "Helvetica", FontSize → 14}, AxesStyle → Arrowheads[Automatic]]
```

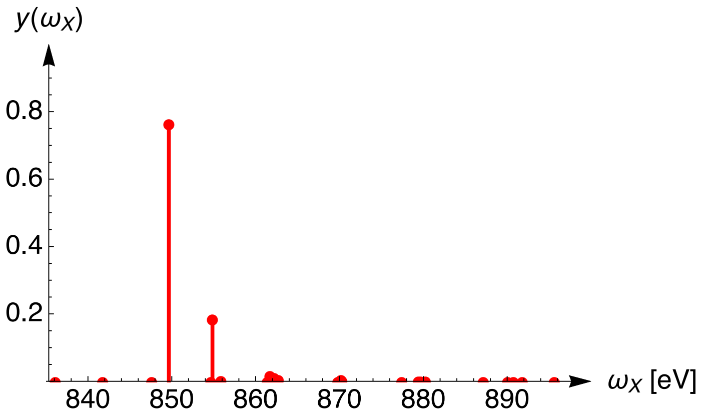


```
spectrumFluorescenceStates = Table[
   {i, fluorescencetransitions[[i]], fluorecenceenergy[[i]] * HartreeToeV, xraySpectrumFluorescenceNorm[[i, 2]]}, {i, 1, 100}];
```

```
Sort[spectrumFluorescenceStates, #1[[4]] > #2[[4]] &][[1 ;; 20]] // TableForm
```

| | | | | |
|---|---|---|---|---|
| 2 | 1s(1) 2s(2) 2p(6) ⟶ 1s(2) 2s(2) 2p(5) | 849.65 | 0.764751 |
| 6 | 1s(1) 2s(2) 2p(5) ⟶ 1s(2) 2s(2) 2p(4) | 854.849 | 0.18467 |
| 15 | 1s(1) 2s(2) 2p(4) ⟶ 1s(2) 2s(2) 2p(3) | 861.711 | 0.0179417 |
| 17 | 1s(1) 2s(1) 2p(5) ⟶ 1s(2) 2s(1) 2p(4) | 862.214 | 0.0109422 |
| 20 | 1s(1) 2s(0) 2p(6) ⟶ 1s(2) 2s(0) 2p(5) | 862.711 | 0.00498038 |
| 29 | 1s(1) 2s(2) 2p(3) ⟶ 1s(2) 2s(2) 2p(2) | 870.192 | 0.00479309 |
| 31 | 1s(1) 2s(1) 2p(4) ⟶ 1s(2) 2s(1) 2p(3) | 870.171 | 0.00396194 |
| 8 | 1s(1) 2s(1) 2p(6) ⟶ 1s(2) 2s(1) 2p(5) | 855.868 | 0.00271629 |
| 34 | 1s(1) 2s(0) 2p(5) ⟶ 1s(2) 2s(0) 2p(4) | 870.276 | 0.00177229 |
| 47 | 1s(1) 2s(1) 2p(3) ⟶ 1s(2) 2s(1) 2p(2) | 879.7 | 0.000686983 |
| 11 | 1s(0) 2s(2) 2p(6) ⟶ 1s(1) 2s(2) 2p(5) | 946.736 | 0.000682672 |
| 50 | 1s(1) 2s(0) 2p(4) ⟶ 1s(2) 2s(0) 2p(3) | 879.407 | 0.000535669 |
| 45 | 1s(1) 2s(2) 2p(2) ⟶ 1s(2) 2s(2) 2p(1) | 880.245 | 0.000306275 |
| 63 | 1s(1) 2s(1) 2p(2) ⟶ 1s(2) 2s(1) 2p(1) | 890.758 | 0.00025892 |
| 90 | 1s(1) 2s(0) 2p(1) ⟶ 1s(2) 2s(0) 2p(0) | 915.795 | 0.000258508 |
| 66 | 1s(1) 2s(0) 2p(3) ⟶ 1s(2) 2s(0) 2p(2) | 890.066 | 0.000231565 |
| 22 | 1s(0) 2s(2) 2p(5) ⟶ 1s(1) 2s(2) 2p(4) | 953.636 | 0.000150796 |
| 89 | 1s(1) 2s(1) 2p(0) ⟶ 1s(2) 2s(0) 2p(0) | 906.634 | 0.000129141 |
| 80 | 1s(1) 2s(0) 2p(2) ⟶ 1s(2) 2s(0) 2p(1) | 902.212 | 0.0000641737 |
| 61 | 1s(1) 2s(2) 2p(1) ⟶ 1s(2) 2s(2) 2p(0) | 891.819 | 0.0000533928 |

## FWHM diameter of the LCLS beam: 18 μm

FWHM of the crater profile:

```
rhoXx := 18 * MicrometerToBohr
rhoYy := rhoXx
```

```
xraySpectrumFluorescenceNorm = photonyields[pulseenergy];
```

```
ListPlot[xraySpectrumFluorescenceNorm, PlotRange → {{835, 900}, {0, 1}}, Filling → Bottom,
 FillingStyle → Thick, PlotMarkers → {Automatic, Small}, PlotStyle → {Red, Thick}, AxesLabel → {"ωX [eV]", "y(ωX)"},
 LabelStyle → {FontFamily → "Helvetica", FontSize → 14}, AxesStyle → Arrowheads[Automatic]]
```

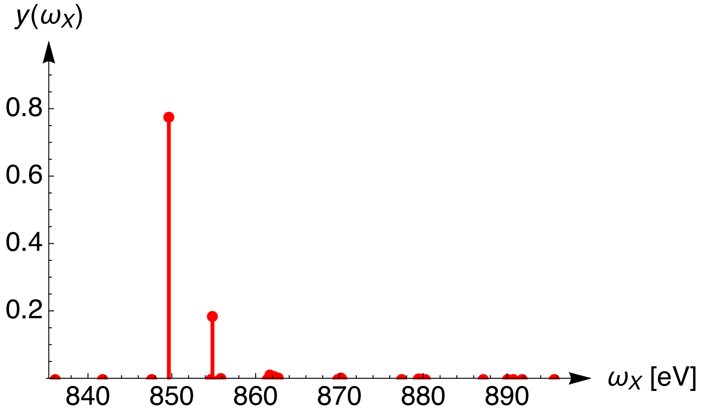


```
spectrumFluorescenceStates = Table[
   {i, fluorescencetransitions[[i]], fluorecenceenergy[[i]] * HartreeToeV, xraySpectrumFluorescenceNorm[[i, 2]]}, {i, 1, 100}];
```

```
Sort[spectrumFluorescenceStates, #1[[4]] > #2[[4]] &][[1 ;; 20]] // TableForm
```

| | | | | | | | | | |
|---|---|---|---|---|---|---|---|---|---|
| 2 | 1s(1) | 2s(2) | 2p(6) | ⟶ | 1s(2) | 2s(2) | 2p(5) | 849.65 | 0.777345 |
| 6 | 1s(1) | 2s(2) | 2p(5) | ⟶ | 1s(2) | 2s(2) | 2p(4) | 854.849 | 0.187298 |
| 15 | 1s(1) | 2s(2) | 2p(4) | ⟶ | 1s(2) | 2s(2) | 2p(3) | 861.711 | 0.0127858 |
| 17 | 1s(1) | 2s(1) | 2p(5) | ⟶ | 1s(2) | 2s(1) | 2p(4) | 862.214 | 0.00780662 |
| 20 | 1s(1) | 2s(0) | 2p(6) | ⟶ | 1s(2) | 2s(0) | 2p(5) | 862.711 | 0.00355975 |
| 29 | 1s(1) | 2s(2) | 2p(3) | ⟶ | 1s(2) | 2s(2) | 2p(2) | 870.192 | 0.00340406 |
| 31 | 1s(1) | 2s(1) | 2p(4) | ⟶ | 1s(2) | 2s(1) | 2p(3) | 870.171 | 0.00278505 |
| 8 | 1s(1) | 2s(1) | 2p(6) | ⟶ | 1s(2) | 2s(1) | 2p(5) | 855.868 | 0.00194341 |
| 34 | 1s(1) | 2s(0) | 2p(5) | ⟶ | 1s(2) | 2s(0) | 2p(4) | 870.276 | 0.00124916 |
| 11 | 1s(0) | 2s(2) | 2p(6) | ⟶ | 1s(1) | 2s(2) | 2p(5) | 946.736 | 0.000484575 |
| 47 | 1s(1) | 2s(1) | 2p(3) | ⟶ | 1s(2) | 2s(1) | 2p(2) | 879.7 | 0.000341709 |
| 50 | 1s(1) | 2s(0) | 2p(4) | ⟶ | 1s(2) | 2s(0) | 2p(3) | 879.407 | 0.000266603 |
| 45 | 1s(1) | 2s(2) | 2p(2) | ⟶ | 1s(2) | 2s(2) | 2p(1) | 880.245 | 0.000152409 |
| 63 | 1s(1) | 2s(1) | 2p(2) | ⟶ | 1s(2) | 2s(1) | 2p(1) | 890.758 | 0.000127354 |
| 66 | 1s(1) | 2s(0) | 2p(3) | ⟶ | 1s(2) | 2s(0) | 2p(2) | 890.066 | 0.000113818 |
| 22 | 1s(0) | 2s(2) | 2p(5) | ⟶ | 1s(1) | 2s(2) | 2p(4) | 953.636 | 0.00010673 |
| 90 | 1s(1) | 2s(0) | 2p(1) | ⟶ | 1s(2) | 2s(0) | 2p(0) | 915.795 | 0.0000884391 |
| 89 | 1s(1) | 2s(1) | 2p(0) | ⟶ | 1s(2) | 2s(0) | 2p(0) | 906.634 | 0.0000443395 |
| 61 | 1s(1) | 2s(2) | 2p(1) | ⟶ | 1s(2) | 2s(2) | 2p(0) | 891.819 | 0.0000264803 |
| 80 | 1s(1) | 2s(0) | 2p(2) | ⟶ | 1s(2) | 2s(0) | 2p(1) | 902.212 | 0.0000222046 |

## FWHM diameter of the LCLS beam: 20 μm

FWHM of the crater profile:

```
rhoXx := 20 * MicrometerToBohr
rhoYy := rhoXx
```

```
xraySpectrumFluorescenceNorm = photonyields[pulseenergy];
```

```
ListPlot[xraySpectrumFluorescenceNorm, PlotRange → {{835, 900}, {0, 1}}, Filling → Bottom,
 FillingStyle → Thick, PlotMarkers → {Automatic, Small}, PlotStyle → {Red, Thick}, AxesLabel → {"ωX [eV]", "y(ωX)"},
 LabelStyle → {FontFamily → "Helvetica", FontSize → 14}, AxesStyle → Arrowheads[Automatic]]
```

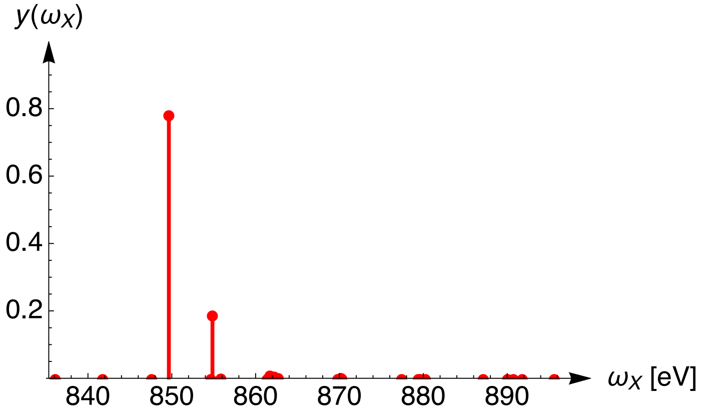


```
spectrumFluorescenceStates = Table[
   {i, fluorescencetransitions[[i]], fluorecenceenergy[[i]] * HartreeToeV, xraySpectrumFluorescenceNorm[[i, 2]]}, {i, 1, 100}];
```

```
Sort[spectrumFluorescenceStates, #1[[4]] > #2[[4]] &][[1 ;; 20]] // TableForm
```

| | | | | |
|---|---|---|---|---|
| 2 | 1s(1) 2s(2) 2p(6) ⟶ 1s(2) 2s(2) 2p(5) | 849.65 | 0.782829 |
| 6 | 1s(1) 2s(2) 2p(5) ⟶ 1s(2) 2s(2) 2p(4) | 854.849 | 0.188437 |
| 15 | 1s(1) 2s(2) 2p(4) ⟶ 1s(2) 2s(2) 2p(3) | 861.711 | 0.0104726 |
| 17 | 1s(1) 2s(1) 2p(5) ⟶ 1s(2) 2s(1) 2p(4) | 862.214 | 0.00639739 |
| 20 | 1s(1) 2s(0) 2p(6) ⟶ 1s(2) 2s(0) 2p(5) | 862.711 | 0.00291949 |
| 29 | 1s(1) 2s(2) 2p(3) ⟶ 1s(2) 2s(2) 2p(2) | 870.192 | 0.00278403 |
| 31 | 1s(1) 2s(1) 2p(4) ⟶ 1s(2) 2s(1) 2p(3) | 870.171 | 0.00226746 |
| 8 | 1s(1) 2s(1) 2p(6) ⟶ 1s(2) 2s(1) 2p(5) | 855.868 | 0.00159456 |
| 34 | 1s(1) 2s(0) 2p(5) ⟶ 1s(2) 2s(0) 2p(4) | 870.276 | 0.0010182 |
| 11 | 1s(0) 2s(2) 2p(6) ⟶ 1s(1) 2s(2) 2p(5) | 946.736 | 0.000396231 |
| 47 | 1s(1) 2s(1) 2p(3) ⟶ 1s(2) 2s(1) 2p(2) | 879.7 | 0.000227202 |
| 50 | 1s(1) 2s(0) 2p(4) ⟶ 1s(2) 2s(0) 2p(3) | 879.407 | 0.00017731 |
| 45 | 1s(1) 2s(2) 2p(2) ⟶ 1s(2) 2s(2) 2p(1) | 880.245 | 0.000101356 |
| 22 | 1s(0) 2s(2) 2p(5) ⟶ 1s(1) 2s(2) 2p(4) | 953.636 | 0.0000871615 |
| 63 | 1s(1) 2s(1) 2p(2) ⟶ 1s(2) 2s(1) 2p(1) | 890.758 | 0.0000842638 |
| 66 | 1s(1) 2s(0) 2p(3) ⟶ 1s(2) 2s(0) 2p(2) | 890.066 | 0.0000752838 |
| 90 | 1s(1) 2s(0) 2p(1) ⟶ 1s(2) 2s(0) 2p(0) | 915.795 | 0.00004743 |
| 89 | 1s(1) 2s(1) 2p(0) ⟶ 1s(2) 2s(0) 2p(0) | 906.634 | 0.0000238164 |
| 61 | 1s(1) 2s(2) 2p(1) ⟶ 1s(2) 2s(2) 2p(0) | 891.819 | 0.0000175843 |
| 80 | 1s(1) 2s(0) 2p(2) ⟶ 1s(2) 2s(0) 2p(1) | 902.212 | 0.0000119673 |

# References


[1] Christian Buth, Ji-Cai Liu, Mau Hsiung Chen, James P. Cryan, Li Fang, James M. Glownia, Matthias Hoener, Ryan N. Coffee, Nora Berrah, *Ultrafast absorption of intense x rays by nitrogen molecules*, J. Chem. Phys. **136**, 214310 (2012), http://dx.doi.org/10.1063/1.4722756.

[2] Y. Hikosaka, T. Kaneyasu, P. Lablanquie, F. Penent, E. Shigemasa, K. Ito, *Multiple Auger decay of the neon 1s-core-hole state studied by multielectron coincidence spectroscopy*, Phys. Rev. A **92**, 033413 (2015), http://dx.doi.org/10.1103/PhysRevA.92.033413.

[3] N. Saito, I. H. Suzuki, *Shake-off processes in photoionization and Auger transition for rare gases irradiated by soft X-rays*, Phys. Scr. **49**, 80–85 (1994), http://dx.doi.org/10.1088/0031-8949/49/1/011.
